# Supplementary material for: Optimizing Recursive Queries with Program Synthesis
Source: arXiv:2202.10390 source file (2022-02-21)
Supplement: Supplementary file 2 [file appendix-magic-alt.tex]

\section{Examples}

%%%%%%%%%%%%%%%%%%%%%%%%%%%%%%%%%%%%%%%%%%%%%%%%%%%%%%%%%%%%%%%%

\remy{We should be able to adapt the proof in Appendix C to this style of proofs, if that's beneficial.
It can also be helpful to have a big commutative diagram to tie together all the steps below.}
We begin by defining the following programs. 
On the left, $\Pi$ is the original unoptimized program.
On the right is a program with two strata, $\Pi_o'$ and $\Pi_o$.
Note all the rules $r_{n-o}$ together form the 
 magic set-optimized program. 
Each rule $r_{n-\texttt{copy}}$ is the same as a rule $r_{n-o}$, 
 except that every relation symbol with subscript $o$, $A_o$, 
 is replaced by a relation symbol with subscript $\texttt{copy}$,
 $A_{\texttt{copy}}$ (primed relations do not change). 
{\small 
$$
\begin{array}{rrrl|rrrl}
    \Pi:
    & r_{1}: & R(x) \cd & V(x) & 
    \Pi_o':
    & r_{1-{o}}: & Q'_{o}() \cd &\\
    & r_{2}: & R(x) \cd & T(x, y, z) \wedge R(y) \wedge R(z) &
    & r_{2-{o}}: & R'_{o}(y) \cd & R'_{o}(x) \wedge T(x,y,z)\\
    & r_{3}: & Q(x) \cd & G(x) \wedge R(x) &
    & r_{3-{o}}: & R'_{o}(z) \cd & R'_{o}(x) \wedge T(x,y,z) \wedge R_{\texttt{copy}}(y)\\
    &&&&
    & r_{4-{o}}: & R'_{o}(x) \cd & Q'_{o}() \wedge G(x)\\
    &&&&\\
    &&&&
    & r_{5-{\texttt{copy}}}: & R_{\texttt{copy}}(x) \cd & R'_{o}(x) \wedge V(x)\\
    &&&&
    & r_{6-{\texttt{copy}}}: & R_{\texttt{copy}}(x) \cd & R'_{o}(x) \wedge
    T(x, y, z) \wedge R_{\texttt{copy}}(y) \wedge R_{\texttt{copy}}(z)\\
    &&&&
    & r_{7-{\texttt{copy}}}: & Q_{\texttt{copy}}(x) \cd & Q'_{o}() \wedge G(x) \wedge R_{\texttt{copy}}(x)\\
    &&&&\\
    &&&&\Pi_o:
    & r_{5-{o}}: & R_{o}(x) \cd & R'_{o}(x) \wedge V(x)\\
    &&&&
    & r_{6-{o}}: & R_{o}(x) \cd &
    R'_{{o}}(x) \wedge T(x, y, z) \wedge R_{o}(y) \wedge R_{o}(z)\\
    &&&&
    & r_{7-{o}}: & Q_{o}(x) \cd &
    Q'_{o}() \wedge G(x) \wedge R_{o}(x)
\end{array}
$$}
The following hold at the least fix point of $\Pi_o'$:
\begin{align}
  \Rightarrow & Q'_{\texttt{o}}() & 
  \forall x: R_{o}'(x) \wedge V(x) \Rightarrow & R_{\texttt{copy}}(x)
  \label{eq:appendix:nnewfixpoint:1}\\
  \forall x,y,z: R'_{\texttt{o}}(x) \wedge T(x,y,z)\Rightarrow & R'_{\texttt{o}}(y) 
  & \forall x,y,z:R'_{\texttt{o}}(x) \wedge T(x,y,z) \wedge R_{\texttt{copy}}(y) \wedge R_{\texttt{copy}}(z)  \Rightarrow & R_{\texttt{copy}}(x)
  \label{eq:appendix:nnewfixpoint:2}\\
  \forall x,y,z:R'_{\texttt{o}}(x) \wedge T(x,y,z) \wedge R_{\texttt{copy}}(y)  \Rightarrow & R'_{\texttt{o}}(z)
  & \forall x: G(x) \wedge Q_o'() \wedge R_{\texttt{copy}}(x) \Rightarrow &  Q_{\texttt{copy}}(x)
  \label{eq:appendix:nnewfixpoint:3}\\
  \forall x: G(x) \wedge Q'_{\texttt{o}}() \Rightarrow & R'_{\texttt{o}}(x)
  \label{eq:appendix:nnewfixpoint:4}
\end{align}
Using the above programs we define the following functions $F, G$ and $H$, 
 where $F$ and $H$ correspond to the ICO of $\Pi$ and $\Pi_o$ respectively:
\begin{align*}
  F(R,Q) = & 
  (\bar R, \bar Q) \mbox{ where: } &
  \bar R(x) = & V(x) \vee \exists y \exists z\left(T(x, y, z) \wedge R(y) \wedge R(z)\right)\\
 && \bar Q(x) = &G(x) \wedge R(x) \\
  H(R_{\texttt{o}}, Q_{\texttt{o}}) = & 
  (\bar R_{\texttt{o}}, \bar Q_{\texttt{o}}) \mbox{ where: }&
  \bar R_{\texttt{o}}(x) = & \left(R'_{\texttt{o}}(x) \wedge V(x)\right) \vee \left(R'_{\texttt{o}}(x) \wedge\exists y \exists z\left(T(x, y, z) \wedge R_{\texttt{o}}(y) \wedge R_{\texttt{o}}(z)\right)\right)\\
 && \bar Q_{\texttt{o}}(x) = & Q'_{\texttt{o}}() \wedge G(x) \wedge R_{\texttt{o}}(x) \\
  G(R,Q) = & 
  (R_{\texttt{aux}},Q_{\texttt{aux}}) \mbox{ where: }&
  R_{\texttt{aux}}(x) = & R'_{\texttt{o}}(x) \wedge R(x) \\
 && Q_{\texttt{aux}}(x) = & Q'_{\texttt{o}}() \wedge Q(x)
\end{align*}
Before we check the \fgh-rule, we first establish an invariant about the function $F$. 
Fix $R_o'$ and $R_{\texttt{copy}}$ to be the relations at the least fix point of $\Pi_o'$,
 then the following is an invariant for $F$ on $R$ (its first input and first output):
\begin{align}
  \forall x :R'_{\texttt{o}}(x) \wedge R(x) \Rightarrow  R_{\texttt{copy}}(x)
\label{eq:appendix:ih:0}
\end{align}
\begin{proof}
  Assume Eq.~\eqref{eq:appendix:ih:0} holds on $R$, 
  we show it also holds on $\bar{R}$ where $F(R, Q) = (\bar R, \bar Q)$ 
  for some $Q$ and $\bar Q$:
  \begin{align*}
    & R_o'(x) \wedge \bar R(x) \\
    & = \mbox{ (by definition of $F$) } \\
    & R_o'(x) \wedge V(x) \vee R_o'(x) \wedge \exists y \exists z\left(T(x, y, z) \wedge R(y) \wedge R(z)\right) \\
    & \Rightarrow \mbox{ (apply Eq.~\eqref{eq:appendix:nnewfixpoint:1}-right)} \\
    & R_{\texttt{copy}}(x) \vee R_o'(x) \wedge \exists y \exists z\left(T(x, y, z) \wedge R(y) \wedge R(z)\right) \\
    & = \mbox{ (apply Eq.~\eqref{eq:appendix:nnewfixpoint:2}-left)} \\
    & R_{\texttt{copy}}(x) \vee \exists y \exists z\left(R_o'(x) \wedge T(x, y, z) \wedge R_o'(y) \wedge R(y) \wedge R(z)\right) \\
    & \Rightarrow \mbox{ (apply Eq.~\eqref{eq:appendix:ih:0})} \\
    & R_{\texttt{copy}}(x) \vee \exists y \exists z\left(R_o'(x) \wedge T(x, y, z) \wedge R_{\texttt{copy}}(y) \wedge R(z)\right) \\
    & = \mbox{ (apply Eq.~\eqref{eq:appendix:nnewfixpoint:3}-left)} \\
    & R_{\texttt{copy}}(x) \vee \exists y \exists z\left(R_o'(x) \wedge T(x, y, z) \wedge R_{\texttt{copy}}(y) \wedge R_o'(z) \wedge R(z)\right) \\
    & \Rightarrow \mbox{ (apply Eq.~\eqref{eq:appendix:ih:0})} \\
    & R_{\texttt{copy}}(x) \vee \exists y \exists z\left(R_o'(x) \wedge T(x, y, z) \wedge R_{\texttt{copy}}(y) \wedge R_{\texttt{copy}}(z)\right) \\
    & \Rightarrow \mbox{ (apply Eq.~\eqref{eq:appendix:nnewfixpoint:2}-right)} \\
    & R_{\texttt{copy}}(x) 
  \end{align*}
\end{proof}
Now we are ready to check the \fgh-rule. The composition $G\circ F$ and $H \circ G$ are as follows:
\begin{align*}
  G(F(R,Q)) = & (R_{\texttt{GF}},Q_{\texttt{GF}}) &\mbox{where: } 
        R_{\texttt{GF}}(x) = &R'_{\texttt{o}}(x) \wedge \left(V(x) \vee \exists y \exists z\left(T(x, y, z) \wedge R(y) \wedge R(z)\right)\right)
  % \label{eq:gf:appendix:1}
  \\
    & & Q_{\texttt{GF}}(x) = &  Q'_{\texttt{o}}() \wedge G(x)\wedge R(x)
  % \label{eq:gf:appendix:2}
  \\
  H(G(R,Q)) = & (R_{\texttt{HG}},Q_{\texttt{HG}}) &\mbox{where: } 
        R_{\texttt{HG}}(x)=& \left(R'_{\texttt{o}}(x) \wedge V(x) \right) \vee \left(R'_{\texttt{o}}(x) \wedge \exists y \exists z\left(T(x, y, z) \wedge R'_{\texttt{o}}(y) \wedge R(y) \wedge R'_{\texttt{o}}(z) \wedge R(z)\right)\right)
  % \label{eq:gf:appendix:3}
  \\
    & & Q_{\texttt{HG}}(x) = & Q'_{\texttt{o}}() \wedge G(x) \wedge R'_{\texttt{o}}(x) \wedge R(x)
  % \label{eq:gf:appendix:4}
\end{align*}

\begin{proof}
  To show $Q_{\texttt{GF}} = Q_{\texttt{HG}}$, simply chase $R_{\texttt{GF}}$ with Eq.~\eqref{eq:appendix:nnewfixpoint:4}.
We now show $R_{\texttt{GF}} = R_{\texttt{HG}}$ by chasing both expressions:
\begin{align*}
  & R_{\texttt{GF}} \\
  & = \mbox{ (by definition)} \\
  & R'_{\texttt{o}}(x) \wedge \left(V(x) \vee \exists y \exists z\left(T(x, y, z) \wedge R(y) \wedge R(z)\right)\right) \\
  & = \mbox{ (chase with Eq.~\eqref{eq:appendix:nnewfixpoint:2}-left)} \\
  & R'_{\texttt{o}}(x) \wedge V(x) \vee \exists y \exists z\left(R'_{\texttt{o}}(x) \wedge T(x, y, z) \wedge R_o'(y) \wedge R(y) \wedge R(z)\right) \\
  & = \mbox{ (chase with Eq.~\eqref{eq:appendix:ih:0})} \\
  & R'_{\texttt{o}}(x) \wedge V(x) \vee \exists y \exists z\left(R'_{\texttt{o}}(x) \wedge T(x, y, z) \wedge R_o'(y) \wedge R(y) \wedge R_{\texttt{copy}}(y) \wedge R(z)\right) \\
  & = \mbox{ (chase with Eq.~\eqref{eq:appendix:nnewfixpoint:3}-left)} \\
  & R'_{\texttt{o}}(x) \wedge V(x) \vee \exists y \exists z\left(R'_{\texttt{o}}(x) \wedge T(x, y, z) \wedge R_o'(y) \wedge R(y) \wedge R_{\texttt{copy}}(y) \wedge R_o'(z) \wedge R(z)\right) \\
  & = \mbox{ (chase with Eq.~\eqref{eq:appendix:ih:0} to remove } R_{\texttt{copy}}(y)) \\
  & R'_{\texttt{o}}(x) \wedge V(x) \vee \exists y \exists z\left(R'_{\texttt{o}}(x) \wedge T(x, y, z) \wedge R_o'(y) \wedge R(y) \wedge R_o'(z) \wedge R(z)\right) \\
  & = \mbox{ (by definition)} \\
  & R_{\texttt{HG}}
\end{align*}
\end{proof}
The \fgh-rule allows us to conclude $G(F^{\omega}(\emptyset, \emptyset)) = H^{\omega}(G(\emptyset, \emptyset))$.
Since $G(\emptyset, \emptyset) = (\emptyset, \emptyset)$ and $G$ does not change $Q$ (because $Q'() = \texttt{true}$), 
we may conclude $F^{\omega}(\emptyset, \emptyset)$ and $H^{\omega}(\emptyset, \emptyset)$ output the same relation $Q$.
It remains to show that the concatenation of $\Pi_o'$ and $\Pi_o$, whose ICO is $H$,
 is equivalent to the magic set-optimized program consisting of only the rules $r_{n-o}$ 
 (with $r_{n-\texttt{copy}}$ removed).
We show that with the following lemma: 
\begin{lemma}\label{appendix:lemma:copy}
  Let $F_1(X_1,X_2, X_{2-\texttt{copy}}), F_2(X_1,X_2)$ be two functions, returning the
  same types as $X_1$ and as $X_2$ respectively.  Then the following
  two programs compute the same $X_1, X_2$ under the invariant $X_{2-\texttt{copy}}=X_2$:

  \begin{align*}
    \Pi_1:\texttt{output } (X_1, X_2, X_{2-\texttt{copy}})
    &&X_1 \cd & F_1(X_1, X_{2-\texttt{copy}}) \\
    &&X_{2-\texttt{copy}} \cd & F_2(X_1, X_{2-\texttt{copy}}) \\
    &&X_2 \cd & F_2(X_1, X_2)
  \end{align*}
  and
  \begin{align*}
    \Pi_2:\texttt{output } (X_1, X_2, X_2)
    &&Y_1 \cd & F_1(Y_1, Y_2) \\
    &&Y_2 \cd & F_2(Y_1, Y_2)
  \end{align*}
\end{lemma}

\begin{proof}
  Define the following function $G$ and invariant $\Psi$:
  \begin{align*}
    G(X_1, X_{2-\texttt{copy}}, X_2) = & (X_1, X_2)\\
    \Psi(X_1, X_{2-\texttt{copy}}, X_2) \equiv & X_{2-\texttt{copy}}=X_2
  \end{align*}
  The followgin can be checked immediately: (1) $\Psi$ is an invariant
  for $\Pi_1$ and (2) under the assumption $\Psi$, the FGH rule holds:
  \begin{align*}
    G(F_1(X_1, X_{2-\texttt{copy}}), F_2(X_1,X_{2-\texttt{copy}}),  F_2(X_1,X_2)) =&(F_1(X_1, X_{2-\texttt{copy}}),F_2(X_1,X_2))\\
    (F_1,F_2)(G(X_1,X_{2-\texttt{copy}},X_2))= (F_1,F_2)(X_1,X_2) = & (F_1(X_1,X_2),F_2(X_1,X_2)
  \end{align*}
  and their equality follows from $\Psi$.
\end{proof}

Notice that program $\Pi_1$ can be stratified: we can compute
$X_1, X_{2-\texttt{copy}}$ in the first stratum, then use their
results as EDBs and compute $X_2$ in the second stratum.

We apply Lemma~\ref{appendix:lemma:copy} to $H$, where $X_1$ is all the primed relations, 
$X_2$ is all the unprimed relations with subscript $o$, and $X_{2-\texttt{copy}}$ is 
all the unprimed relations with subscript $\texttt{copy}$.
This shows $H$ computes the same results as the magic set-optimized program, 
 therefore the optimized program computes the same $Q$ as the original program.

\reinhard{This proof of first establishing the invariant in Eq. 40 (via an application of the FGH-rule) and then proving $R_o = R'_o \wedge R$ with another application of the FGH-rule looks great! It is much more elegant than the proof in 
Appendix C. And above all, it completely avoids the problems with inflationary vs.\ non-inflationary ICO by considering  $R_{2\texttt{copy}}$ and $R'_o$ (the analogue of $M'_{\calO}$) as EDBs.
\\
Interestingly, while the proof (of the $\subseteq$-part) in Appendix C had 2 induction proofs, now we actually have even 3 induction proofs: \\
*) implicitly in the proof of Eq. 40: over the number of ICO-applications for $R(x)$\\
*) nested inside the first induction proof:  over the IDB-atoms in the rule body \\
*) in the proof of the property $R_o = R'_o \wedge R$: again over the IDB-atoms in the rule body 
}

%%%%%%%%%%%%%%%%%%%%%%%%%%%%%%%%%%%%%%%%%%%%%%%%%%%%%%%%%%%%%%%%

\clearpage
\section*{Continuation of Appendix D}

%%%%%%%%%%%%%%%%%%%%%%%%%%%%%%%%%%%%%%%%%%%%%%%%%%%%%%%%%%%%%%%%
\eat{
\begin{example}
  \label{ex:hung}  A simple  non-linear query:
  \begin{align*}
    \Pi_P:
    &r_1: & R(x) \cd &  V(x)\\
    &r_2: & R(x) \cd & T(x, y, z) \wedge R(y) \wedge R(z)\\
    &r_3: & Q(x) \cd & R(x) \wedge G(x)
  \end{align*}
  The adorment is $R^+, Q^-$, and the optimized query is:
  \begin{align*}
    \Pi_O:
    &r_4: & Q'() \cd & \\
    &r_5: & R'(y) \cd & R'(x) \wedge T(x,y,z) & \mbox{item~\ref{item:def:magicsets:1} applied to rule $r_2$ and atom $R(y)$} \\
    &r_6: & R'(z) \cd & R'(x) \wedge T(x,y,z) \wedge R(y)  & \mbox{item~\ref{item:def:magicsets:1} applied to rule $r_2$ and atom $R(z)$} \\
    &r_7: & R'(x) \cd & Q'() \wedge G(x)   & \mbox{item~\ref{item:def:magicsets:1} applied to rule $r_3$ and atom $R(x)$} \\
    &r_1': & R(x) \cd & R'(x) \wedge V(x)\\
    &r_2': & R(x) \cd & R'(x) \wedge T(x, y, z) \wedge R(y) \wedge R(z)\\
    &r_3': & Q(x) \cd & Q'() \wedge R(x) \wedge G(x)
  \end{align*}

  We start by computing $M_O'$, followed by $T_{\tilde O}(M_O')$

  \begin{align*}
    \Pi_1:
    &r_4: & Q'() \cd & \\
    &r_5: & R'(y) \cd & R'(x) \wedge T(x,y,z) & \mbox{item~\ref{item:def:magicsets:1} applied to rule $r_2$ and atom $R_{\texttt{temp}}(y)$} \\
    &r_6: & R'(z) \cd & R'(x) \wedge T(x,y,z) \wedge R_{\texttt{temp}}(y)  & \mbox{item~\ref{item:def:magicsets:1} applied to rule $r_2$ and atom $R_{\texttt{temp}}(z)$} \\
    &r_7: & R'(x) \cd & Q'() \wedge G(x)   & \mbox{item~\ref{item:def:magicsets:1} applied to rule $r_3$ and atom $R_{\texttt{temp}}(x)$} \\
    &r_1'': & R_{\texttt{temp}}(x) \cd & R'(x) \wedge V(x)\\
    &r_2'': & R_{\texttt{temp}}(x) \cd & R'(x) \wedge T(x, y, z) \wedge R_{\texttt{temp}}(y) \wedge R_{\texttt{temp}}(z)\\
    &r_3'': & Q_{\texttt{temp}}(x) \cd & Q'() \wedge R_{\texttt{temp}}(x) \wedge G(x) \\
    & & & & \mbox{NEW STRATUM} \\
    &r_1': & R_{\texttt{opt}}(x) \cd & R'(x) \wedge V(x)\\
    &r_2': & R_{\texttt{opt}}(x) \cd & R'(x) \wedge T(x, y, z) \wedge R_{\texttt{opt}}(y) \wedge R_{\texttt{opt}}(z)\\
    &r_3': & Q_{\texttt{opt}}(x) \cd & Q'() \wedge R_{\texttt{opt}}(x) \wedge G(x)
  \end{align*}

  {\bf Part 1} of the proof.  We show that $\Pi$ is ``equivalent'' to
  the second stratum above, where $R'$ is now an EDB computed by the
  first stratum.  More precisely:

  \begin{align*}
    F(R,Q) = & (R_{\texttt{new}},Q_{\texttt{new}}) & \mbox{where: }R_{\texttt{new}}(x)  = &   V(x) \vee \exists y \exists z (T(x, y, z) \wedge R(y) \wedge R(z))\\
             &    & Q_{\texttt{new}}(x) = & R(x) \wedge G(x)\\
    H(R_{\texttt{opt}},Q_{\texttt{opt}}) = & (R_{\texttt{opt-new}},Q_{\texttt{opt-new}})  & \mbox{where: } R_{\texttt{opt-new}}(x)  = &   R'(x) \wedge \left(V(x) \vee \exists y \exists z (T(x, y, z) \wedge R_{\texttt{opt}}(y) \wedge R_{\texttt{opt}}(z))\right)\\
             &    & Q_{\texttt{opt-new}}(x) = & Q'() \wedge R_{\texttt{opt-new}}(x) \wedge G(x)\\
   G(R,Q) = & (R_{\texttt{opt}},Q_{\texttt{opt}}) & \mbox{where: } R_{\texttt{opt}}(x) = & R(x) \wedge R'(x) \\
            &         & Q_{\texttt{opt}}(x) = & Q(x) \wedge Q'()
  \end{align*}

  We prove:
  \begin{align*}
    G(F(R,Q)) = & (R_{\texttt{opt-new}}, Q_{\texttt{opt-new}})  & \mbox{where: } R_{\texttt{opt-new}}(x) = & R'(x) \wedge (V(x) \vee \exists y \exists z (T(x, y, z) \wedge R(y) \wedge R(z)))\\
                &      & Q_{\texttt{opt-new}}(x) = & Q'() \wedge R(x) \wedge G(x)\\
    \\
    H(G(R,Q)) = & (R_{\texttt{opt-new}}, Q_{\texttt{opt-new}})  & \mbox{where: } R_{\texttt{opt-new}}(x) =&R'(x) \wedge (V(x) \vee \exists y \exists z (T(x, y, z) \wedge R'(y)\wedge R(y)\wedge R'(z) \wedge R(z)))\\
   & & Q_{\texttt{opt-new}}(x) = & Q'() \wedge R'(x) \wedge R(x) \wedge G(x)
  \end{align*}

  We use the following properties of $R'$ and $R$:
  \begin{align*}
    \forall x, y, z: R'(x) \wedge T(x,y,q) \Rightarrow & R'(y) \\
    \forall x, y, z: R'(x) \wedge T(x,y,q) \wedge R_{\texttt{temp}}(y) \Rightarrow & R'(z) \\
    \forall x: R(x) \Rightarrow & R_{\texttt{temp}}(x)
  \end{align*}
  The first two implications state that $R'$ is a minimal model of
  magic set rules.

  The third implications should be an invariant of the program $\Pi$,
  asserting that $R$ remains a subset of the minimal model
  $R_{\texttt{temp}}$.  \yell{Problem here, this is not true}
  
   This proves that the following two programs:
   \begin{align*}
     \Pi_1:
     &r_1: & R(x) \cd &  V(x)\\
     &r_2: & R(x) \cd & T(x, y, z) \wedge R(y) \wedge R(z)\\
     &r_3: & Q(x) \cd & R(x) \wedge G(x)
   \end{align*}
   \begin{align*}
     \Pi_2':
     &r_1: & R_{\texttt{opt}}(x) \cd &  V(x)\\
     &r_2: & R_{\texttt{opt}}(x) \cd & R'(x) \wedge T(x, y, z) \wedge R_{\texttt{opt}}(y) \wedge R_{\texttt{opt}}(z)\\
     &r_3: & Q_{\texttt{opt}}(x) \cd & Q'() \wedge R_{\texttt{opt}}(x) \wedge G(x)
   \end{align*}
   are ``equivalent'', in the following precise way:
   \begin{align*}
     R_{\texttt{opt}}(x) = & R'(x) \wedge R(x) & Q_{\texttt{opt}}(x) = & Q'() \wedge Q(x)
   \end{align*}
\end{example}
}
%%%%%%%%%%%%%%%%%%%%%%%%%%%%%%%%%%%%%%%%%%%%%%%%%%%%%%%%%%%%%%%%

\begin{example}
  Consider the reverse-same-generation program:
  \begin{align*}
    r_1: &&  S(x,y) \cd & E(x,y) \\
    r_2: &&  S(x,y) \cd & U(x,p) \wedge S(q,p) \wedge D(y,q) \\
    r_3: &&  Q_1(y) \cd & S(a,y)
  \end{align*}
  To help the reader keep track of the transformations below, we have
  separated the edges into ``up edges'' denoted $U(x,p)$, ``down
  edges'' denoted $D(y,q)$, and horizontal edges denoted $E(x,y)$.
  Our discussion applies immediately to the case when $U=D=E$.  We
  describe here how to derive the magic-set optimized program as a
  sequence of ``modding'' or ``adorments''.

  The first step is create two copies of $S$, the left $Sl$ and the
  right $Sr$.  More precisely, consider the program:
  \begin{align*}
    r_4: && Sl(x,y) \cd & E(x,y) \\
    r_5: && Sr(x,y) \cd & E(x,y) \\
    r_6: && Sl(x,y) \cd & U(x,p)\wedge Sr(q,p) \wedge D(y,q) \\
    r_7: && Sr(x,y) \cd & U(x,p)\wedge Sl(q,p) \wedge D(y,q) \\
    r_8: && Q_2(y) \cd & Sl(a,y)
  \end{align*}

  We prove that new program is equivalent to the previous and, for
  that, we will use the following notation.  If $r, r', \ldots$ are
  rules and $R, R', \ldots$ are relation names, then
  $\Pi(r, r', \ldots; R,R',\ldots)$ denotes the program consisting of
  these rules that returns only the IDB predicates $R, R', \ldots$.
  In this notation the two programs above are $\Pi(r_1,r_2,r_3; Q_1)$
  and $\Pi(r_4,r_5,r_6,r_7,r_8; Q_2)$ respectively.

\begin{proposition}
  $\Pi(r_1,r_2; S,S) \equiv \Pi(r_4,r_5,r_6,r_7; Sl,Sr)$.
\end{proposition}
In other words, if we run rules $r_1, r_2$ and return the pair $(S,S)$
we obtain the same result as running rules $r_4, \ldots, r_7$ and
returning $(Sl,Sr)$.

\begin{proof}
  We use the FGH rule.  The three functions are:
  \begin{align*}
    F(S)\defeq & S' &&\mbox{ where}& S'(x,y)\defeq & E(x,y) \vee \exists p,q(U(x,p) \wedge S(q,p) \wedge D(y,q))\\
    G(S)\defeq & (Sl,Sr) &&\mbox{ where}& Sl(x,y) = Sr(x,y) \defeq & S(x,y)\\
    H(Sl,Sr) \defeq & (Sl',Sr') &&\mbox{ where}& Sl'(x,y)\defeq & E(x,y) \vee \exists p,q(U(x,p) \wedge Sr(q,p) \wedge D(y,q))\\
               &           &&             & Sr'(x,y)\defeq & E(x,y) \vee \exists p,q(U(x,p) \wedge Sl(q,p) \wedge D(y,q))
  \end{align*}
  It is immediate to check that $G(F(S)) = H(G(S))$.
\end{proof}

\begin{corollary}
  $\Pi(r_1,r_2,r_3; Q_1) \equiv \Pi(r_4,r_5,r_6,r_7,r_8; Q_2)$
\end{corollary}

Next, we adorn the IDBs $Sl, Sr, Q_2$ as follows:
$Sl^{+-}, Sr^{-+}, Q_2^-$.  Recall that we are also allowed to reorder
the atoms in each rule: we chose to reorder those in the rule for
$Sr^{-+}$.  The program now becomes:

\begin{align*}
  r_4: && Sl^{+-}(x,y) \cd & E(x,y) \\
  r_5: && Sr^{-+}(x,y) \cd & E(x,y) \\
  r_6: && Sl^{+-}(x,y) \cd & U(x,p)\wedge Sr^{-+}(q,p) \wedge D(y,q) \\
  r_7: && Sr^{-+}(x,y) \cd & D(y,q) \wedge Sl^{+-}(q,p) \wedge U(x,p) \\
  r_8: && Q_2^-(y) \cd & Sl^{+-}(a,y)
\end{align*}

Next, we apply the transformations in Def.~\ref{def:magicsets} and
obtain:

\begin{align*}
  \mbox{item~\ref{item:def:magicsets:1} on $r_6$}: && Sr'(p) \cd & Sl'(x)\wedge U(x,p) \\
  \mbox{item~\ref{item:def:magicsets:1} on $r_7$}: && Sl'(q) \cd & Sr'(y)\wedge D(y,q) \\
  \mbox{item~\ref{item:def:magicsets:1} on $r_8$}: && Sl'(a) \cd & Q_2'()\\
  \mbox{item~\ref{item:def:magicsets:2}}: && Q_2'() \cd &\\
  \mbox{item~\ref{item:def:magicsets:3} on $r_4$}: && Sl^{+-}(x,y) \cd & Sl'(x)\wedge E(x,y) \\
  \mbox{item~\ref{item:def:magicsets:3} on $r_5$}: && Sr^{-+}(x,y) \cd & Sr'(y) \wedge E(x,y) \\
  \mbox{item~\ref{item:def:magicsets:3} on $r_6$}: && Sl^{+-}(x,y) \cd &Sl'(x)\wedge U(x,p)\wedge Sr^{-+}(q,p) \wedge D(y,q) \\
  \mbox{item~\ref{item:def:magicsets:3} on $r_7$}: && Sr^{-+}(x,y) \cd &Sr'(y)\wedge D(y,q) \wedge Sl^{+-}(q,p) \wedge U(x,p) \\
  \mbox{item~\ref{item:def:magicsets:3} on $r_8$}: && Q_2^-(y) \cd & Q_2'(),Sl^{+-}(a,y)
\end{align*}
\end{example}
