# Supplementary material for: Optimizing Recursive Queries with Program Synthesis
Source: arXiv:2202.10390 source file (2022-02-21)
Supplement: Supplementary file 3 [file appendix-magic-new.tex]

\clearpage

\section{Magic Set Optimization}
% \label{app:magic:sets}

\newcommand{\au}{\mathtt{aux}}
\newcommand{\fgh}{\textrm{FGH}}

\newcommand{\barR}{\bar{R}}

\newcommand{\progO}{\Pi_O}
\newcommand{\progP}{\Pi}
\newcommand{\progA}{\Pi_{aux}}
\newcommand{\progOne}{\Pi_{aux}^1}
\newcommand{\progTwo}{\Pi_{aux}^2}
\newcommand{\progPQ}{\progP \cup \{r_Q\}}
\newcommand{\progOQ}{\progO \cup \{r_Q\}}
\newcommand{\progAQ}{\progA \cup \{r_Q\}}

\newcommand{\RP}{\mathcal{R}_{P}}
\newcommand{\RPi}{\mathcal{R}_{\progP}}
\newcommand{\RPtwo}{\mathcal{R}_{\progTwo}}
\newcommand{\bodyr}{\mathit{body}_r}
\newcommand{\bodyrtilde}{\mathit{body}_{\tilde r}}

\newcommand{\TP}{T_{\progP}}
\newcommand{\MP}{M_{\progP}}

\newcommand{\MO}{M_{\progO}}
\newcommand{\MA}{M_{\progA}}
\newcommand{\MOne}{M_{\progOne}}
\newcommand{\MTwo}{M_{\progTwo}}

\newcommand{\MPQ}{M_{\progPQ}}
\newcommand{\MOQ}{M_{\progOQ}}
\newcommand{\MAQ}{M_{\progAQ}}

\newcommand{\fl}{\mathtt{flat}}
\newcommand{\up}{\mathtt{up}}

\newcommand{\sg}{\mathtt{sg}}

\newcommand{\sgbf}{\mathtt{sg^{bf}}}
\newcommand{\sgp}{\mathtt{sg'}}
\newcommand{\isgbf}{\mathtt{input\_sg^{bf}}}

In \cite{DBLP:conf/birthday/MascellaniP02}, Mascellani and Pedreschi presented a
very elegant correctness proof of the magic set optimization of logic programs. Its main
characteristics are:

\begin{enumerate}
\item applying a declarative style rather than the usual procedural reasoning;
\item allowing arbitrary ``modings'' (i.e., designating input and
output positions in each relation) rather than adornments, which are
usually used to trace the binding of variables in each rule body; and
\item adopting an iterative approach -- considering a single moding at a time rather than
all possible adornments at once.
\end{enumerate}

In this section, we present a correctness proof of
the magic set optimization based on our \fgh-framework. 
This proof takes some inspiration from the one of  \cite{DBLP:conf/birthday/MascellaniP02}. In particular, 
we will also use modings and adopt a declarative style. Moreover, some terminology and notation will be 
borrowed from 
\cite{DBLP:conf/birthday/MascellaniP02}.

\paragraph*{\bf Notation}
As in \cite{DBLP:conf/birthday/MascellaniP02}, we use upper case letters $A,B, \dots $ to denote single atoms in a datalog rule and bold face letters $\bA, \bB, \dots$ to denote a (possibly empty) sequence of atoms. Datalog rules are thus of the form
$A \cd \bA$. For given program $\progP$, we write $\MP$ to denote the minimal model of $\progP$ (or, equivalently, the lfp of the 
ICO of program $\progP$). It is sometimes convenient to
consider $\MP$ as a set of
ground atoms rather than a collection of relations.
For the formulation of datalog queries, we follow the 
convention used in \cite{DBLP:books/aw/AbiteboulHV95}: a query is given by a datalog program $\Pi$ and 
a query predicate $Q$ not occurring in $\progP$, such that $Q$ is defined
by a single rule $r_Q$ of the form 
$r_Q : Q(\bv)  \cd R(\ba,\bv)$. That is, the head atom consists of pairwise distinct variables $\bv$ and the body consists of a single atom in which some of the arguments may be a (possibly empty)  
vector $\ba$ of constants. 
As in \cite{DBLP:conf/birthday/MascellaniP02},
we write $[Q]$ to denote the set of all possible ground instances of $Q$.

\paragraph*{\bf Modes}
For an $n$-ary relation symbol $R$, a {\em mode\/} for $R$ is a function
$$
m_R \colon \{1, \dots, n\} \rightarrow \{+,-\}
$$
with the understanding that $m_R(i) = +$ (respectively  $m_R(i) = -$) means that
$i $ is an input (respectively output) position of $R$.
A more intuitive notation of the moding of a relation symbol
$R$ is in the form $R(m_R(1), \dots, m_R(n))$. In  \cite{DBLP:conf/birthday/MascellaniP02}, this notation is
illustrated by the example $\mathtt{sum}(+,+,-)$, where $\mathtt{sum}$ is a predicate that takes two numbers as input and produces their sum in the third component.

In the sequel, we will assume some fixed moding for
a given program. W.l.o.g., we may assume that, for every relation symbol,
the input positions precede the output positions. Hence, an atom $A$ is of the form $R(\mathbf{u}, \mathbf{v})$ with
input arguments $\mathbf{u}$ and output arguments~$\mathbf{v}$.

\paragraph*{\bf Magic set optimization}
For an atom $A$ of the form $R(\mathbf{u}, \mathbf{v})$, we denote the {\em magic version\/} of $A$ as $A' = R'(\mathbf{u})$
for some fresh predicate symbol $R'$. (Recall that we assume a fixed mode for every relation symbol $R$ in a given program).
Recall that we are assuming 
the query predicate $Q$ to be defined
by a single rule of the form 
$Q(\bv)  \cd R(\ba,\bv)$, where $\ba$ is a vector of constants.
While the moding may be arbitrarily chosen for 
all other predicates, the 
moding of $R$ must be such that the input positions
are precisely the positions of the constant-arguments $\ba$. Hence, the ``magic version'' of $R(\ba,\bv)$ is the ground atom $R'(\ba)$.

Then the magic set transformation can be defined as follows (cf.\ \cite{DBLP:conf/birthday/MascellaniP02}, Definition~3):

\begin{definition}
\label{def:magicsets}
Consider a program $\progP$ together with  
query predicate $Q$. The magic program $\progO$ is obtained from $\progP$ by the
following transformation steps:

\begin{enumerate}
\item \label{item:def:magicsets:1} For every rule $r \colon A \cd \bA$ (with fixed order of the body atoms) of $\progP$,
and every IDB atom $B$ in the body of $r$,
let $\bB$ denote the sequence of body atoms
to the left of $B$ and let $\bC$ denote the sequence of body atoms
to the right of $B$, i.e., the rule body $\bA$ is of the form
$\bB, B, \bC$. Then we add a new rule
$B' \cd A', \bB$ to the program;
\item \label{item:def:magicsets:2} 
Let the query predicate be defined by the 
rule $Q(\bv)  \cd R(\ba,\bv)$. Then 
add a new single-atom rule $R'(\ba) \cd$ ;
\item \label{item:def:magicsets:3} replace each original rule $A \cd \bA$ from $\progP$ by
the new rule $A \cd A', \bA$.
\end{enumerate}
The rule 
$r_Q : Q(\bv) \cd R(\ba,\bv)$ 
defining the query predicate $Q$ is left unchanged.
\end{definition}
As is noted in \cite{DBLP:conf/birthday/MascellaniP02}, the notion of ``modes'' is more general than that of the usual
adornments resulting from a bound/free analysis.
The usual magic set optimization is obtained  by
first introducing appropriate copies of each 
IDB predicate (these copies correspond to the different adornments to be considered for each predicate) 
and then imposing 
different modings on these copies (these modings 
capture the corresponding adornments). The correctness of
the magic set transformation is stated as follows (cf.\ \cite{DBLP:conf/birthday/MascellaniP02}, Theorem 4):

\begin{theorem}
\label{theo:magicsets}
Let $\progP$ be a datalog program with 
query predicate $Q$ by the rule $r_Q$, 
and let $\progO$ be the corresponding magic program. Then
the following property holds:
$$
\MPQ \cap [Q] = \MOQ \cap [Q]
$$
\end{theorem}

In other words, the two programs yield the same answer tuples for query $Q$.

\paragraph*{\bf Correctness proof of the magic set optimization}
We introduce an ``intermediate'' program $\progA$ for which we will establish the equivalence (in terms of query $Q$) with both, the original program $\progP$ and the optimized program $\progO$. 
Intuitively, this intermediate program $\progA$ 
splits the magic set optimization in two steps, corresponding to 
two strata of $\progA$: 
first, it computes the magic sets via copies of the 
the original IDB predicates; then it computes the
restricted IDB relations by adding the magic atoms to the rule bodies. 

Formerly, for every IDB atom $A = R(\mathbf{u}, \mathbf{v})$ in $\progP$, we define 
$A_{\texttt{copy}} = R_{\texttt{copy}}(\mathbf{u}, \mathbf{v})$ for a fresh predicate symbol $R_{\texttt{copy}}$. 
For a sequence $\bA$ of atoms, we write 
$\bA_{\texttt{copy}}$ to denote the sequence of atoms obtained by taking $\bA$ and replacing every IDB atom $A$ in $\bA$ by $A_{\texttt{copy}}$. 
Then we define $\progA$ with two strata
$\progOne$ and $\progTwo$ as follows:

% \remy{Minor: would it be simpler to say $\mathbf{\progOne}$ is the magic program 
% but with every IDB $R$ replaced by $R_\texttt{copy}$?}
\medskip
\noindent
$\mathbf{\progOne}$:
\begin{enumerate}
\item \label{item:def:intermediate:1} For every rule $r \colon A \cd \bA$ (with fixed order of the body atoms) of $\progP$,
and every IDB atom $B$ in the body of $r$,
let $\bB$ denote the sequence of body atoms
to the left of $B$ and let $\bC$ denote the sequence of body atoms
to the right of $B$, i.e., the rule body $\bA$ is of the form
$\bB, B, \bC$. Then we add a new rule
$B' \cd A', \bB_{\texttt{copy}}$ to the program;
\item \label{item:def:intermediate:2} 
Let the query predicate be defined by the 
rule $Q(\bv)  \cd R(\ba,\bv)$. Then 
add a new single-atom rule 
$R'_{\texttt{copy}}(\ba) \cd$ ;
\item \label{item:def:intermediate:3} 
For every rule $r \colon A \cd \bA$  of $\progP$,
add the rule $A_{\texttt{copy}} \cd A', \bA_{\texttt{copy}}$.
\end{enumerate}
$\mathbf{\progTwo}$:
\begin{enumerate}
\setcounter{enumi}{3}
\item \label{item:def:intermediate:4} 
For every rule $r \colon A \cd \bA$ of $\progP$,
add the rule $A \cd A', \bA$.
\end{enumerate}
Again, the rule $r_Q : Q(\bv) \cd R(\ba,\bv)$ defining the query predicate $Q$ is left unchanged.

\smallskip

Note that $\progOne$ is simply the magic program $\progO$ but with every IDB $R$ replaced by $R_\texttt{copy}$. Program $\progA$ is clearly stratified. Hence, when evaluating 
the second stratum $\progTwo$, we may assume all predicates occurring in $\progOne$ as EDBs. It is therefore allowed to consider $\progTwo$ as a datalog program by itself and,
for instance, talk about the ICO of program $\progTwo$
(which will play a crucial role in the correctness proof 
of the magic set optimization below).

By considering the model-theoretic semantics of datalog (i.e., interpreting each datalog rule as a universally quantified implication), we observe that  
the following invariants hold for the least fixpoint of the first stratum 
$\progOne$ of $\progA$: 

\begin{align}
  \forall \bx : \bA  \Rightarrow & A 
  & \mbox{for every rule  $A \cd \bA$ with variables
  $\bx$ in program $\progOne$}
  \label{eq:appendix:tgd:1}
\end{align}

Note that, following the three cases in the definition of 
program $\progOne$, we thus get three kinds of invariants: 
%
% \remy{``all arguments of $Q'$ are ground'' where do we assume this?
% Do we need to restrict the moding to conclude this?}
%
\begin{enumerate}
\item \label{item:def:tgd:1} For every rule $r \colon A \cd \bA$ of $\progP$,
and every IDB atom $B$ in the body of $r$,
let $\bx$ denote the variables in $r$, 
let $\bB$ denote the sequence (or, equivalently, the conjunction) 
of body atoms to the left of $B$.
% and let $\bC$ denote the sequence of body atoms to the right of $B$. 
Then the invariant 
$\forall \bx : A' \wedge \bB_{\texttt{copy}} \Rightarrow B'$ holds 
in the lfp of $\progOne$.
\item \label{item:def:tgd:2} 
Let the query predicate be defined by the 
rule $Q(\bv)  \cd R(\ba,\bv)$. Then 
the invariant 
$\Rightarrow R'(\ba)$ holds in the lfp of $\progOne$. 
In other words, the ground atom $R'(\ba)$ is (trivially) contained 
in the lfp of $\progOne$.
\item \label{item:def:tgd:3} 
For every rule $A \cd \bA$ from $\progP$ with 
variables  $\bx$, 
the 
invariant $\forall \bx : A' \wedge \bA_{\texttt{copy}} 
\Rightarrow A_{\texttt{copy}}$ holds
in the lfp of $\progOne$. 
\end{enumerate}

\smallskip

% \remy{Minor: ``program $P$ with $P \in \{\progP, \progOne, \progTwo\}$''
% $\progTwo$ is a valid program only if the magic predicates are EDBs.}
\paragraph*{\bf Further Notation}
It is convenient to introduce the following notation
to simplify the presentation of what follows: for EDB predicate $R$, we set $R' := R$ (which is consistent
with the idea that EDB-predicates consist of input positions only) and 
also $R_{\texttt{copy}} := R$. Moreover, for IDB predicate $R$
of program $P$ with $P \in \{\progP, \progOne, \progTwo\}$, 
we define $\RP(R)$  as the set of rules in program $P$
with head predicate $R$. 
W.l.o.g., we assume that all these rules have the same head atom 
$R(\bx)$, where $\bx$ is a set (or vector) of pairwise distinct variables.
Suppose that $\progP$ (and, hence, also $\progTwo$) has $m$ IDB 
predicates $(R_1, \dots, R_m)$. 
Then, for a rule $r$, we write $\bodyr(S_1, \dots, S_m)$
to denote the conjunction of atoms resulting from taking the body of $r$ and replacing each atom $R_j$ by $S_j$. 
By slight abuse of notation, a predicate name $R$ may be used to denote either the predicate or a relation for this predicate. Finally, it is convenient to 
consider the body of a rule interchangeably
either as a sequence of atoms or as a conjunction of 
atoms. 

% \remy{Minor: ``a useful invariant that holds between programs $\progP$
% and $\progA$'' strictly speaking the invariant is only on $\progP$, 
% although it does involve relations computed by $\progA$.}
Before we prove the equivalence of $\progP$ and $\progA$ in terms of 
query $Q$, we establish 
a useful invariant that holds during the evaluation of $\progP$, assuming that 
$\progOne$ has already been fully evaluated:

\begin{lemma}
Let $\progP$ be a datalog program, 
and let stratum $\progOne$ of program
$\progA$ be as defined above,
and let $R$ be an IDB predicate in $\progP$. Moreover, let 
$R(\mathbf{u}, \mathbf{v})$ be the atom obtained by putting 
pairwise distinct variables $\mathbf{u}, \mathbf{v}$ 
in the input and output positions of $R$. Then the following 
invariant holds during the evaluation of program $\progP$, 
in case $\progOne$ has already been fully evaluated:
\begin{align}
  \forall \mathbf{u} \forall \mathbf{v} :R'(\mathbf{u}) \wedge 
        R(\mathbf{u},\mathbf{v}) \Rightarrow  R_{\texttt{copy}}(\mathbf{u},\mathbf{v})
\label{eq:appendix:tgd:2}
\end{align}
\end{lemma}

\begin{proof}[Proof of invariant~\eqref{eq:appendix:tgd:2}]
The proof is by induction on the number of iterations of the ICO $F$ of 
program $\progP$. Clearly, after 0 iterations, relation 
$R$ is empty and the implication holds trivially. 
For the induction step, assume that 
eq.~\eqref{eq:appendix:tgd:2} holds after $n$ iterations of the ICO $F$.
Moreover, suppose that the IDB-relations 
in $F^n(\emptyset, \dots, \emptyset)$ are $(R_1, \dots, R_m)$. 
Then, in the next iteration of $F$, 
$\progP$ produces the following relations:

     \begin{align*}
       F(R_1, \dots, R_m) = & 
       (\barR_1, \dots \barR_m) &\mbox{where: \quad } 
       \barR_i (\bu,\bv)  = &
       \bigvee_{r \in \RPi(R_i)} 
       \exists \by_r :
       \bodyr(R_1, \dots, R_m)
       \mbox{ with $\by_r = var(\bodyr) \setminus (\bu \cup \bv)$}       
     \end{align*}

\noindent
That is, $\barR_i (\bu,\bv)$ is generated by some rule $r$ in 
$\progP$ with head predicate $R_i$.
We have to show, for every $i \in \{1, \dots, m \}$,
that the implication 
$\forall \bu \forall \bv : R'_i(\bu) \wedge \barR_i(\bu,\bv) \Rightarrow R_{i-\texttt{copy}}(\bu,\bv)$
holds. 
By the above expansion of $F(R_1, \dots, R_m)$, we have 
$$R'_i(\bu) \wedge \barR_i (\bu,\bv)  = 
       \bigvee_{r \in \RPi(R_i)} 
       \exists \by_r :  R'_i(\bu) \wedge  \bodyr(R_1, \dots, R_m)
       \mbox{ with $\by_r = var(\bodyr) \setminus (\bu \cup \bv)$}       
$$
Consider an arbitrary rule $r \in  \RPi(R_i)$. 
Then $\bodyr(R_1, \dots, R_m)$ is of the form 
$S_1(\bx_1) \wedge \dots \wedge S_\ell(\bx_\ell)$.
We claim that the following implication holds: 
$$\forall \bx : R'_i(\bu) \wedge S_1(\bx_1) \wedge \dots \wedge S_\ell(\bx_\ell)
\Rightarrow 
S_{1-\texttt{copy}}(\bx_1) \wedge \dots \wedge  S_{\ell-\texttt{copy}}(\bx_\ell)
\mbox{ with } \bx = \bu \cup \bx_1 \cup \dots \cup \bx_\ell
$$
From this, we derive the desired implication~\eqref{eq:appendix:tgd:2} 
as follows: 
$\progP$ contains the rule
$r$ with  $r \colon R_i(\bu,\bv) \cd S_1(\bx_1) \wedge \dots \wedge S_\ell(\bx_\ell)$.
Hence, by our construction,
program $\progOne$ contains the rule 
$R_{i-\texttt{copy}}(\bu,\bv) \cd R'_i(\bu), 
S_{1-\texttt{copy}}(\bx_1), \dots, S_{\ell-\texttt{copy}}(\bx_\ell)$.
Hence, the invariants~\eqref{eq:appendix:tgd:1} contain the implication
$\forall \bx : R'_i(\bu) \wedge 
S_{1-\texttt{copy}}(\bx_1) \wedge \dots \wedge S_{\ell-\texttt{copy}}(\bx_\ell)
\Rightarrow R_{i-\texttt{copy}}(\bu,\bv)$.
Therefore, if we manage to prove the above claim, then it follows that 
the presence of $R_{i}(\bu,\bv)$ in $F(R_1, \dots, R_m)$ together with 
$R'_u(\bu)$ in the lfp of $\progOne$ indeed implies the presence of 
$R_{i-\texttt{copy}}(\bu,\bv)$ in the lfp of $\progOne$.
It remains to prove the claim.

\smallskip
\noindent
{\em Proof of the claim.} In order to prove the implication
$$ \forall \bx : R'_i(\bu) \wedge S_1(\bx_1) \wedge \dots \wedge S_\ell(\bx_\ell)
\Rightarrow 
S_{1-\texttt{copy}}(\bx_1) \wedge \dots \wedge  S_{\ell-\texttt{copy}}(\bx_\ell)
$$
we show, for every $j \in \{1, \dots, \ell\}$, 
that the following implication holds:
$$ \forall \bx : 
R'_i (\bu) \wedge S_1(\bx_1) \wedge \dots \wedge S_\ell(\bx_\ell) 
\Rightarrow
S'_j (\bu_j) \wedge S_{j-\texttt{copy}} (\bx_j)
$$
%
% \remy{I had missed that this part is actually inductive in my proof,
% and the following is very clear!}
We prove this property by induction on $j$. 
Note that the implication of the atom $S'_j (\bu_j) $ is only needed for the induction proof.
For the induction begin, let $j = 0$ and there is nothing to prove. 
For the induction step, suppose that we have already shown that this property
holds for every $\alpha \in \{1, \dots, j\}$ for $j \geq 0$. 
By our construction, program $\progOne$
contains a rule 
$S'_{\alpha+1} (\bu_{\alpha+1}) \cd 
R'_i(\bu_i), S_{1-\texttt{copy}} (\bx_1), \dots,
S_{\alpha-\texttt{copy}} (\bx_\alpha)$. 
Hence, by the invariants~\eqref{eq:appendix:tgd:1}, 
we may conclude that 
$R'_i(\bu_i), S_{1-\texttt{copy}} (\bx_1), \dots,
S_{\alpha-\texttt{copy}} (\bx_\alpha)$
implies 
$S'_{\alpha+1} (\bu_{\alpha+1})$.
Hence, together with the induction hypothesis (of the induction 
on $j$ ranging over the body atoms of rule $r$), we have: 
$$\forall \bx : 
R'_i (\bu) \wedge S_1(\bx_1) \wedge \dots \wedge S_\ell(\bx_\ell) 
\Rightarrow
R'_i(\bu_i), S_{1-\texttt{copy}} (\bx_1), \dots,
S_{\alpha-\texttt{copy}} (\bx_\alpha)
\Rightarrow
S'_{\alpha+1} (\bu_{\alpha+1})
$$

\noindent
Now we can apply the induction hypothesis (of the
induction on the number $n$ of iterations of the ICO $F$ of
program $\progP$) to 
conclude that 
$ \forall \bx_{\alpha+1} :  S'_{\alpha+1} (\bu_{\alpha+1})\wedge
S_{\alpha+1} (\bx_{\alpha+1}) 
\Rightarrow 
S_{(\alpha+1)-\texttt{copy}} (\bx_\alpha)$
holds and, therefore, in total, also
$$\forall \bx : 
R'_i (\bu) \wedge S_1(\bx_1) \wedge \dots \wedge S_\ell(\bx_\ell) 
\Rightarrow
S_{(\alpha+1)-\texttt{copy}} (\bx_\alpha)
$$
This concludes the proof of the claim and, thus, also the proof of 
invariant~\eqref{eq:appendix:tgd:2} 
\end{proof}

\noindent
We are now ready to prove the equivalence of $\progP$ and $\progA$
in terms of query $Q$.

\begin{proof}[Proof of Theorem \ref{theo:magicsets}]
For both programs, $\progP$ and $\progA$, 
let the query predicate $Q$ to be defined
by the rule $r_Q : Q(\bv)  \cd R(\ba,\bv)$. 
To prove the equivalence of the two programs in terms of $Q$, 
it therefore suffices to show that the following property holds:
$$
\MP \cap [R(\ba,\bv)] = \MA \cap [R(\ba,\bv)]
$$
where $[R(\ba,\bv)]$ denotes the set of all ground instances of 
$R(\ba,\bv)$. Since $\ba$ is a vector of constants, of course, these
positions remain unchanged in every ground instance.

We prove this property via the \fgh-property of the following functions 
$F,G,H$: 
let $F$ be the ICO of program $\progP$ and 
let $H$ be the ICO of program $\progTwo$ -- where we consider the 
relations from the first stratum $\progOne$ as EDBs. 
We thus have $\MA = \MTwo$.
Suppose that $\progP$ contains $m$ IDB predicates
$R_1, \dots, R_m$. 
Then function $G$ maps the $m$-tuple of relations 
$(R_1, \dots, R_m)$ to   
$(R'_1 \cap R_1, \dots, R'_m \cap R_m)$.
To verify that these functions $F,G,H$ satisfy the $\fgh$-property,
we expand the expressions $G(F(R_1, \dots, R_m))$ and 
$H(G(R_1, \dots, R_m))$ and prove their equivalence.

     \begin{align*}
       G(F(R_1, \dots, R_m)) = & 
       (\barR_1, \dots \barR_m) &\mbox{where: \quad } 
       \barR_i (\bu,\bv)  = &
       R'_i(u) \wedge \bigvee_{r \in \RPi(R_i)} \exists \by_r : \bodyr(R_1, \dots, R_m)
       \mbox{ with $\by_r = var(\bodyr) \setminus (\bu \cup \bv)$}
       \\
       H(G(R_1, \dots, R_m)) = & 
       (\barR_1, \dots \barR_m) &\mbox{where: \quad } 
       \barR_i (\bu,\bv)  = &
       \bigvee_{\tilde{r} \in \RPtwo(R_i)} 
       \exists \by_r :
       \bodyrtilde(R'_1 \wedge R_1, \dots, R'_m \wedge R_m)
       \mbox{ with $\by_r = var(\bodyr) \setminus (\bu \cup \bv)$}       
     \end{align*}

\noindent
We have to show that the two ways of computing 
$(\barR_1, \dots \barR_m)$ are equivalent. 
Recall that, by construction, there is a one-to-one correspondence between
the rules $r$ in $\progP$ and $\tilde r$ in $\progTwo$.
Suppose that 
$$\bodyr(R_1, \dots, R_m) = S_1(\bx_1) \wedge \dots \wedge S_\ell(\bx_\ell) 
$$
for rule $r$ with head predicate $R_i$. 
Then 
$$\bodyrtilde(R'_1 \wedge R_1, \dots, R'_m \wedge R_m) = 
R'_i \wedge S'_1(\bu_1) \wedge S_1(\bx_1)
\wedge \dots \wedge S'_\ell(\bu_\ell) \wedge  S_\ell(\bx_\ell). 
$$
In order to prove 
that the two ways of computing 
$(\barR_1, \dots \barR_m)$ are indeed equivalent,
it therefore suffices to show the following equivalence:
$$
R'_i (\bu) \wedge S_1(\bx_1) \wedge \dots \wedge S_\ell(\bx_\ell) 
= 
R'_i (\bu) \wedge
 S'_1(\bu_1) \wedge S_1(\bx_1)
\wedge \dots \wedge S'_\ell(\bu_\ell) \wedge  S_\ell(\bx_\ell)
$$
To this end,
we prove for every $j \in \{1, \dots, \ell\}$ 
that the following implication holds:
$$
R'_i (\bu) \wedge S_1(\bx_1) \wedge \dots \wedge S_\ell(\bx_\ell) 
\Rightarrow
S'_j (\bu_j) \wedge S_{j-\texttt{copy}} (\bx_j)
$$
We prove this property by induction on $j$. 
Note that the implication of the atom $S_{j-\texttt{copy}} (\bx_j)$ 
is only needed for the induction proof.
For the induction begin, let $j = 0$ and there is nothing to prove. 
For the induction step, suppose that we have already shown that this property
holds for every $\alpha \in \{1, \dots, j\}$ for $j \geq 0$. 
By our construction, program $\progOne$
contains a rule 
$S'_{\alpha+1} (\bu_{\alpha+1}) \cd 
R'_i(\bu_i), S_{1-\texttt{copy}} (\bx_1), \dots,
S_{\alpha-\texttt{copy}} (\bx_\alpha)$. 
Hence, by the invariants~\eqref{eq:appendix:tgd:1}, 
we may conclude that 
$R'_i(\bu_i), S_{1-\texttt{copy}} (\bx_1), \dots,
S_{\alpha-\texttt{copy}} (\bx_\alpha)$
implies 
$S'_{\alpha+1} (\bu_{\alpha+1})$.
Hence, together with the induction hypothesis, we have: 

$$\forall \bx :
R'_i (\bu) \wedge S_1(\bx_1) \wedge \dots \wedge S_\ell(\bx_\ell) 
\Rightarrow
R'_i(\bu_i), S_{1-\texttt{copy}} (\bx_1), \dots,
S_{\alpha-\texttt{copy}} (\bx_\alpha)
\Rightarrow
S'_{\alpha+1} (\bu_{\alpha+1})
$$

\noindent
Now we can apply invariant~\eqref{eq:appendix:tgd:2}
to conclude that 
$\forall \bx_{\alpha+1} : S_{\alpha+1} (\bx_{\alpha+1}) \wedge
S'_{\alpha+1} (\bu_{\alpha+1})
\Rightarrow 
S_{(\alpha+1)-\texttt{copy}} (\bx_\alpha)$
holds and, therefore, in total, also
$$\forall \bx : 
R'_i (\bu) \wedge S_1(\bx_1) \wedge \dots \wedge S_\ell(\bx_\ell) 
\Rightarrow
S_{(\alpha+1)-\texttt{copy}} (\bx_\alpha)
$$

\smallskip

The \fgh-rule allows us to conclude 
$G(F^{\omega}(\emptyset, \dots, \emptyset)) = 
H^{\omega}(G(\emptyset, \dots, \emptyset))$.
Moreover, we have $G(\emptyset, \dots, \emptyset) = 
(\emptyset, \dots, \emptyset)$. 
Hence, for every IDB $R_i$ in $\progP$ and $\progTwo$
and every ground atom $R_i(\bc,\bd)$, we have 
$$
R_i(\bc,\bd) \in \MP \Leftrightarrow R'_i(\bc) \in \MOne
\mbox{ and } R_i(\bc,\bd) \in \MTwo
$$
with $\MTwo = \MA$, since we are considering all 
predicates occurring in $\progOne$ as EDBs in $\progTwo$.
Let the query predicate be defined by the 
rule $r_Q :  Q(\bv)  \cd R(\ba,\bv)$.
Atom $R'(\ba)$ is contained in 
the lfp of $\progA$ by invariant~\eqref{eq:appendix:tgd:1}. 
We thus get the desired equivalence 
$$
R(\ba,\bd) \in \MP \Leftrightarrow 
R(\ba,\bd) \in \MA
\mbox{ for every vector $\bd$ of constants} 
$$
and therefore also 
$$
Q(\bd) \in \MPQ \Leftrightarrow 
Q(\bd) \in \MAQ
\mbox{ for every vector $\bd$ of constants} 
$$
\end{proof}

It remains to show that query relation  $Q$ in the lfp of 
program $\progA$ and query relation $Q$ in the lfp of 
the optimized program $\progO$ are also identical. 
We show this with the following lemma: 
\begin{lemma}\label{appendix:lemma:stratification}
  Let $F_1(X_1,X_2, X_{2-\texttt{copy}}), F_2(X_1,X_2)$ be two functions, returning the
  same types as $X_1$ and as $X_2$ respectively.  Then the following
  two programs compute the same $X_1, X_2$ under the invariant $X_{2-\texttt{copy}}=X_2$:

  \begin{align*}
    \Pi_1:\texttt{output } (X_1, X_2, X_{2-\texttt{copy}})
    &&X_1 \cd & F_1(X_1, X_{2-\texttt{copy}}) \\
    &&X_{2-\texttt{copy}} \cd & F_2(X_1, X_{2-\texttt{copy}}) \\
    &&X_2 \cd & F_2(X_1, X_2)
  \end{align*}
  and
  \begin{align*}
    \Pi_2:\texttt{output } (X_1, X_2, X_2)
    &&Y_1 \cd & F_1(Y_1, Y_2) \\
    &&Y_2 \cd & F_2(Y_1, Y_2)
  \end{align*}
\end{lemma}

\begin{proof}
  Define the following function $G$ and invariant $\Psi$:
  \begin{align*}
    G(X_1, X_{2-\texttt{copy}}, X_2) = & (X_1, X_2)\\
    \Psi(X_1, X_{2-\texttt{copy}}, X_2) \equiv & X_{2-\texttt{copy}}=X_2
  \end{align*}
  The following can be checked immediately: (1) $\Psi$ is an invariant
  for $\Pi_1$ and (2) under the assumption $\Psi$, the FGH rule holds:
  \begin{align*}
    G(F_1(X_1, X_{2-\texttt{copy}}), F_2(X_1,X_{2-\texttt{copy}}),  F_2(X_1,X_2)) =&(F_1(X_1, X_{2-\texttt{copy}}),F_2(X_1,X_2))\\
    (F_1,F_2)(G(X_1,X_{2-\texttt{copy}},X_2))= (F_1,F_2)(X_1,X_2) = & (F_1(X_1,X_2),F_2(X_1,X_2)
  \end{align*}
  and their equality follows from $\Psi$.
\end{proof}

Notice that program $\Pi_1$ can be stratified: we can compute
$X_1, X_{2-\texttt{copy}}$ in the first stratum, then use their
results as EDBs and compute $X_2$ in the second stratum.

We apply Lemma~\ref{appendix:lemma:stratification} 
to $H$, where $X_1$ is all the primed relations, 
$X_2$ is all the unprimed relations with subscript $o$, and $X_{2-\texttt{copy}}$ is 
all the unprimed relations with subscript $\texttt{copy}$.
This shows $H$ computes the same results as the magic set-optimized program, 
therefore the optimized program computes the same $Q$ as the original program.

\reinhard{The same-generation example below has to be adapted to the new proof of the magic set optimization. I assume that a few correction cycles will be needed for the proof. I'd therefore like to wait with the adaptation of the example until the  proof has become stable. }

We now illustrate the above formulation of the magic set transformation
and its correctness proof by the ``same-generation'' program.
Suppose that we
are given a graph with
2 kinds of edges $\fl$ (for horizontal connections) and $\up$
(for vertical connections) and that we are interested in all vertices from the
``same generation'' as some given vertex $\mathtt{a}$. Then the program together with
the corresponding query are defined as follows:

\medskip

\noindent
\texttt{Program} $\progP$: \\
$\mathtt{\sg(x,y)}$ :- $\mathtt{\fl(x,y)}$. \\
$\mathtt{\sg(x,y)}$ :- $\mathtt{\up(x,x_1), \sg(x_1,y_1), \up(y,y_1)}$. \\
with single-atom query  $\mathtt{\sg(a,y)}$

\medskip

\noindent
Let us choose the mode $\sg(+,-)$ for the only IDB predicate of the program.
As we will see below, modes for the EDB predicate are irrelevant.
By step 1 of the magic transformation in Definition \ref{def:magicsets}, we get the following rule:

\medskip

\noindent
$\mathtt{\sgp(x_1)}$ :- $\mathtt{\sgp(x), \up(x,x_1)}$.

\medskip

\balance
\noindent
Note that, in principle, step 1 as defined in Definition~\ref{def:magicsets}
(and in \cite{DBLP:conf/birthday/MascellaniP02}) would also produce
rules with head atom $\up'$. However, since EDB atoms never occur in a
rule head, step 3 of the magic transformation would never use a primed
EDB predicate in the body of any rule.
Hence, the primed version of EDB predicates would have
no effect at all on the query atom and can, therefore, safely be omitted.

Now consider step 2 of the magic set transformation in
Definition~\ref{def:magicsets}. It produces the following rule:

\medskip

\noindent
$\mathtt{\sgp(a)}$ :- .

\medskip

Finally, by step 3, we replace the original rules with head predicate
$\sg$ by the following rules:

\medskip

\noindent
$\mathtt{\sg(x,y)}$ :- $\mathtt{\sgp(x), \fl(x,y)}$. \\
$\mathtt{\sg(x,y)}$ :- $\mathtt{\sgp(x),\up(x,x_1), \sg(x_1,y_1), \up(y,y_1)}$.

\medskip

So, in total, we get the following optimized program $\progO$:

\medskip

\noindent
\texttt{Program} $\progO$: \\
$\mathtt{\sgp(x_1)}$ :- $\mathtt{\sgp(x),\up(x,x_1)}$. \\
$\mathtt{\sgp(a)}$ :- .   \\
$\mathtt{\sg(x,y)}$ :- $\mathtt{\sgp(x), \fl(x,y)}$. \\
$\mathtt{\sg(x,y)}$ :- $\mathtt{\sgp(x),\up(x,x_1), \sg(x_1,y_1), \up(y,y_1)}$. \\
with single-atom query  $\mathtt{\sg(a,y)}$

\medskip
\noindent
Note that this is exactly the program that we would get by the usual magic set transformation based on adornments (see e.g., \cite{DBLP:books/aw/AbiteboulHV95})
by considering the adornment $\sgbf$ for the only IDB predicate $\sg$ and renaming
the ``magic predicate'' $\sgp$ to $\isgbf$. Moreover, by way of a minor optimization,
one could define an auxiliary relation $\au$ for the atom sequence  $\mathtt{\sgp(x),\up(x,x_1)}$ to avoid the need to compute this join twice (in the first and last rules above).

\begin{example}
\label{ex:magic:sets}
Suppose that we want to apply the programs $\progP$ and $\progO$ to the graph
$G$ with the following $\fl$ and $\up$ edges:

\bigskip

\begin{center}
\begin{tabular}{c|c}
\multicolumn{2}{c}{$\fl$:} \\
\hline
\texttt{b} & \texttt{e} \\
\texttt{c} & \texttt{f} \\
\texttt{f} & \texttt{c}
\end{tabular}
\hspace{50pt}
\begin{tabular}{c|c}
\multicolumn{2}{c}{$\up$:} \\
\hline
\texttt{a} & \texttt{b} \\
\texttt{a} & \texttt{c} \\
\texttt{b} & \texttt{c} \\
\texttt{d} & \texttt{e} \\
\texttt{e} & \texttt{f}
\end{tabular}
\end{center}

\bigskip

We get the following minimal models of
$\progP$ and $\progO$ over the input database $G$:
{\small
\begin{align*}
    \MP  &= G \cup \{\mathtt{\sg(a,d)},
\mathtt{\sg(a,e)},
\mathtt{\sg(b,e)},
\mathtt{\sg(c,f)},
\mathtt{\sg(d,a)},
\mathtt{\sg(e,b)},
\mathtt{\sg(f,c)}\} \\
\MO &= G \cup \{\mathtt{\sgp(a)},
\mathtt{\sgp(b)}, \mathtt{\sgp(c)},
\mathtt{\sg(a,d)},
\mathtt{\sg(a,e)},
\mathtt{\sg(b,e)}
\mathtt{\sg(c,f)} \}
\end{align*}
} % end of \small
That is, in both cases, the instances of the query atom $\mathtt{\sg(a,y)}$ are
$\{\mathtt{\sg(a,d)},
\mathtt{\sg(a,e)} \}$.

Let us also check one application of the
\fgh-rule. Suppose that we choose $J \subseteq \MP$ with $J = \{
\mathtt{\sg(b,e)}$,
$\mathtt{\sg(c,f)}$,
$\mathtt{\sg(f,c)}$. Note that this would be the result of one application of $\TP$ to the input database $G$. We now verify that, for this set $J$, the equality $g(f(J)) = h(g(J))$ holds. First note that we have $\MO' = \{\mathtt{\sgp(a)},
\mathtt{\sgp(b)},
\mathtt{\sgp(c)}
\}$. Then we get:
\begin{align*}
    J^* &= f(J) = J \cup
    \{\mathtt{\sg(a,d)},\mathtt{\sg(a,f)},
    \mathtt{\sg(e,b)} \} \\
    K^*  &= g(J^*) = \MO' \cup G \cup
    \{\mathtt{\sg(b,e)},\mathtt{\sg(c,f)},
    \mathtt{\sg(a,d)},\mathtt{\sg(a,f)} \} \\
    K  &= g(J) = \MO' \cup G \cup
    \{\mathtt{\sg(b,e)},\mathtt{\sg(c,f)} \\
    K^*  &= h(K) = K \cup
    \{\mathtt{\sg(a,d)},\mathtt{\sg(a,f)} \}
\end{align*}

The two ways of computing $K^*$ as $K^* = g(f(J))$
and as $K^* = h(g(J))$, respectively, yield the same result. Of course, as was shown in the proof of Theorem \ref{theo:magicsets}, this is the case for  any $J$.
\end{example}

\clearpage
