# Supplementary material for: Optimizing Recursive Queries with Program Synthesis
Source: arXiv:2202.10390 source file (2022-02-21)
Supplement: Supplementary file 4 [file appendix.tex]

\section{Data Size}

\begin{center}
\begin{tabular}{c c c}
  Dataset & $|V|$ & $|E|$ \\
  \toprule
  wiki & 7,115 & 103,689 \\
  twitter & 81,306 & 1,768,149 \\
  epinions & 75,879 & 508,837 \\
  \bottomrule
\end{tabular}
\end{center}

For SSSP we convert each graph to a DAG by sorting each edge.

\section{Related Work}
As we discussed, the DeALS family of systems~\cite{DBLP:conf/icde/ShkapskyYZ15}
can express programs optimized by \prem.
However they rely on the programmer to perform the rewrite and
check that \prem\ is applicable.
Our optimizer is automated and supports the more general FGH-rule.

A number of tools exist that leverage SMT-solvers to reason about
query languages~\cite{
  DBLP:conf/cidr/ChuWWC17,
  DBLP:conf/icfem/VeanesGHT09,
  DBLP:conf/cav/GrossmanCIRS17,
  DBLP:journals/pacmpl/0001DLC18,
  DBLP:conf/sosp/SchlaipferRLS17}.
We contribute by proposing a simple and sound encoding that can
be used in \cegis, and works in conjunction with a rewrite system
to reason about semiring operations including unbounded aggregation.

Recent work~\cite{
  DBLP:journals/pvldb/WangSCPD20,
  DBLP:journals/pacmpl/RaghothamanMZNS20,
  DBLP:conf/ijcai/SiRHN19,
  DBLP:conf/cp/AlbarghouthiKNS17,
  DBLP:conf/sigsoft/SiLZAKN18}
has investigated synthesizing Datalog programs.
The specification of the desired program is given by input-output examples.
In comparison, we take a Datalog program as the reference implementation
which completely specifies the semantics of the program to be synthesized.
Unlike prior work which must synthesize recursive definitions,
we leverage the FGH-rule to solve the optimization problem
by synthesizing a non-recursive expression.
The cited papers also propose techniques to speed up \cegis;
since we implement our optimizer atop the general \cegis\ system Rosette,
we can readily benefit from these new techniques when they are
incorporated in Rosette.

\section{Prefix Sum}

\begin{figure}
\fcolorbox{black}{light-gray}{\parbox{0.45\textwidth}{
\footnotesize
  \begin{align*}
    F(P) \defeq & P' &&\mbox{where} & P'(n,i,w) \defeq & [n=i] \wedge V(i,w) \vee \\
    &&&&&[n > i \geq 1] \wedge P(n-1, i, w) \\
    G(P) \defeq & S  &&\mbox{where} & S[n] \defeq & \sum_{i,w} \{ w \mid P(n,j,w) \} \\
    H(S) \defeq & S' &&\mbox{where} & S'[n] \defeq & V[n] + S[n-1]
  \end{align*}
}}
\caption{Expressions $F,G,H$ in Example~\ref{ex:simple:prefix}.}\label{fig:simple:prefix}
\end{figure}

\begin{example}[Prefix Sum]\label{ex:simple:prefix} Consider the following Python program:
  \begin{lstlisting}[language=python]
def p(n): return [v[i] for i in range(n)]
def s(n): return sum(p(n))
  \end{lstlisting}
  which computes the sum of
  the first $n$ elements in the array \texttt{v}. This can be compiled
  to a datalog program:
  \begin{align}
    P(n, i, w) \cd & [n=i] \wedge V(i,w) \vee \nonumber \\
                   & [n > i \geq 1] \wedge P(n-1, i, w). \\
    S[n] \cd & \sum_{i,w} \{ w \mid P(n,j,w) \}.
  \end{align}
  where $P$ is compiled from \texttt{p(n)} which computes
  the $n$-prefix of the array \texttt{v},
  and $S$ is compiled from \texttt{s(n)} which sums over the prefix.
  This verbatim translation stores the $k$-prefix for all $1 \leq k \leq n$
  in $P$, which is wasteful if we only query $S[k]$ for a specific $k$.
  A more efficient datalog program directly computes the sum:
  \begin{align}
    S[n] \cd V[n] + S[n-1].
  \end{align}
  The $F,G,H$ expressions for the two versions of prefix sum are shown in
  Figure~\ref{fig:simple:prefix}.
  One can verify using a tedious but straightforward calculation that
  $G(F(P))=H(G(P))$.
\end{example}

\section{Shortest Paths with Length $\leq$ 10}

How to prove the following: 

\begin{align}
    \bigoplus_{z, w_1, w_2} & [T(x,z,w_1)] \otimes [E(x,y,w_2)] \nonumber \\
    & \otimes w_1 \otimes w_2 \otimes 1_{w_1 \otimes w_2 \leq 10} \\
  = \bigoplus_{z, u_1, u_2} & 1_{u_1 = \bigoplus_{w_1} T(x,z,w_1) \otimes w_1}
                              \otimes 1_{u_2=\bigoplus_{w_2} E(x,y,w_2) \otimes w_2} \nonumber \\
                            & \otimes u_1 \otimes u_2 \otimes 1_{u_1 \otimes u_2 \leq 10} \\
  = \bigoplus_{z, u_{1}} & 1_{u_1 = \bigoplus_{w_1} T(x,z,w_1) \otimes w_1} \nonumber \\
                            & \otimes u_{1} \otimes \bigoplus_{w_2} E(x,y,w_2) \otimes w_2 \nonumber \\
                            & \otimes 1_{u_{1} \otimes \bigoplus_{w_2} E(x,y,w_2) \otimes w_2 \leq 10} \\
  = \bigoplus_{z} & \bigoplus_{w_1} T(x,z,w_1) \otimes w_1 \nonumber \\
                            & \otimes \bigoplus_{w_2} E(x,y,w_2) \otimes w_2 \nonumber \\
                            & \otimes 1_{\bigoplus_{w_1} T(x,z,w_1) \otimes w_1
                              \otimes \bigoplus_{w_2} E(x,y,w_2) \otimes w_2 \leq 10} \\
  = \bigoplus_{z} & \bigoplus_{w_1, w_{2}} T(x,z,w_1) \otimes w_1 \otimes E(x,y,w_2) \otimes w_2 \nonumber \\
                            & \otimes 1_{\bigoplus_{w_1, w_{2}} T(x,z,w_1) \otimes w_1
                              \otimes E(x,y,w_2) \otimes w_2 \leq 10}
\end{align}

\section{From Eval}
\subsection{Datalog Systems}

There is a great number of commercial and open-source datalog engines in the
wild, but only a few support aggregate in recursion. Supporting non-recursive
aggregate is straightforward given any datalog engine: simply create a separate
stratum for the aggregation. Therefore, we only consider one system that lacks
recusive aggregate and use it as a baseline. We were able to identify five
systems that support recursive aggregates:
SociaLite~\cite{DBLP:journals/tkde/SeoGL15},
Myria~\cite{10.14778/2824032.2824052}, the DeALS family of systems
(DeALS~\cite{DBLP:conf/icde/ShkapskyYZ15},
BigDatalog~\cite{DBLP:conf/sigmod/ShkapskyYICCZ16}, and
RaDlog~\cite{DBLP:conf/sigmod/0001WMSYDZ19}),
RecStep~\cite{DBLP:journals/pvldb/FanZZAKP19}, and
Dyna~\cite{francislandau-vieira-eisner-2020-wrla}.

RecStep: ``{\em We allow aggregation not only in non-recursive rules, but inside
recursion as well, as studied in~\cite{DBLP:conf/fgcs/Lefebvre92}. In the latter
case, one must be careful that the semantics of the Datalog program lead to
convergence to a fixpoint; in this paper, we assume that the program given as
input always converges (\cite{DBLP:conf/amw/ZanioloYIDSC18} studies how to test
this property).}'' In short, RecStep provides no guarantee that pushing down
an aggregate preserves program semantics.

The single-threaded implementation of DeALs allows a recursive aggregate if the
programs is {\em premappable}. However, it leaves the responsibility of checking
premappability to the programmer. Our approach can be used to automatically
verify a generalized notion of premappability. All of BigDatalog, RaDlog and
DeALs support monotonic aggregates which does not require premappability.
However, an additional aggregate is usually required to compute the final
output, because monotonic aggregates do not produce unique results. For example,
the program
\[SP_{0}(x, y, \text{mmin}(w_{1} + w_{2})) \text{ :- } E(x,z,w_{1}), SP_{0}(y,z,w_{2}).\]
will collect shortest paths found in every iteration of rule application. That
is, for every $x,y$ there are multiple values of $w$ such that
$(x, y, w) \in SP_{0}$. Therefore we must compute the final result with an
additional aggregate:
\[SP(x,y,\min(w)) \text{ :- } SP_{0}(x, y, w).\]

SociaLite ``{\em supports recursive aggregate functions. We show that
semi-naive evaluation can be applied to recursively-defined aggregate functions,
if they are meet operations and that the rest of the rules are monotonic under
the partial order induced by the meet operations. In addition, taking advantage
of the commutativity of meet operations, we can speed up the convergence of the
solution by prioritizing the evaluation.}'' Restricting the aggregates to meet
operations precludes Sum.

Myria: ``{\em we show that it is possible to recursively evaluate aggregate
functions that are commutative, associative, and bag-monotonic (but not
necessarily idempotent). Examples of bag-monotonic aggregates include Count,
Sum, which are not idempotent, and also include Min and Max.}'' Bag-monotonicity
restricts aggregates to natural numbers in Myria, whereas we support summation
over the reals as seen in the sliding-window sum example.

Dyna defines the semantics of its programs using {\em bag relations}, and
supports recursive aggregates in a similar fashion to Myria. Dyna forgoes many
restrictions commonly found in datalog dialects and is Turing-complete. To avoid
non-termination when possible, it does not use the traditional relational
operations like join and union to execute a program; instead its interpreter is
implemented as a {\em rewrite system}. The rewrite system applies a set of
carefully designed rewrite rules to simplify a program-query pair to some normal
form. The rewrite rules include some of the algrbraic identities we use in our
optimizer, and therefore Dyna can perform some of the rewrites we discover. But
because Dyna's execution model is idiosyncratic, a rewrite that speeds up in a
relational engine may make a Dyna program slower.

Overall, we are aware of no existing system that can automatically perform all
of our aggregate-pushdown optimizations while guaranteeing correctness.
Furthermore, we can perform a range of other optimizations including rewriting
the non-monotone sliding-window sum, inverting recursion, and optimizations
under constraints. \remy{We can pushdown the recusion in MLM if the input is a
tree; we can also remove the aggregate in APSP if the input is a tree. Tree-ness
can be expressed as a key constraint. }

\subsection{Benchmark Programs}
\subsubsection{Graph Analytics}
\remy{Need to make casts explicit.}
\begin{lstlisting}[language=prolog]
  /* all-pair shortest paths */
  %% naive definition
  P(x,y,w):-E(x,y,w).
  P(x,y,w):-E(x,z,w1),P(z,y,w2),w=w1+w2.
  SP[x,y]=min[w:P(x,y,w)+w].
  %% optimized program
  SP[x,y]=min(min[w:E(x,y,w)+w],
              min[y:SP[x,y]+
                    min[w:E(x,y,w)+w]]).
\end{lstlisting}

\begin{lstlisting}[language=prolog]
  /* reachability */
  %% naive definition
  TC(x,y):-E(x,y).
  TC(x,y):-E(x,z),TC(z,y).
  R(y):-TC(1,y).
  %% optimized program
  R(y):-E(1,y).
  R(y):-R(x),E(x,y).
\end{lstlisting}

\begin{lstlisting}[language=prolog]
  /* betweennes centrality */
  %% naive definition
  C[s,v]=sum[t:D[s,t]=D[s,v]+D[v,t]*
               sig[s,v]*sig[v,t]/
               sig[s,t]].
  %% optimized program
  C[s,v]=sum[t:E(v,t)*D[s,t]=D[s,v]+1*
               sig[s,v]/sig[s,t]*
               (1+C[s,t])].
\end{lstlisting}

\begin{lstlisting}[language=prolog]
  /* connected components */
  %% naive definition
  TC(x,y):-E(x,y).
  TC(x,y):-E(x,z),TC(z,y).
  CC[x]=min[y:TC(x,y)+y].
  %% optimized program
  CC[x]=min(V(x)+x,
            min[y:min(cc[y],E(y,x)+x)]).
\end{lstlisting}

\subsubsection{Statistics}

\begin{lstlisting}[language=prolog]
  /* prefix sum */
  %% naive definition
  R(t,j,w):-v(j,w),t=j.
  R(t,j,w):-R(t-1,j,w),1<=j<t.
  P[t]=sum[j,w:R(t,j,w)*w].
  %% optimized program
  P[t]=v[t]+P[t-1].
\end{lstlisting}

\begin{lstlisting}[language=prolog]
  /* sliding window sum */
  %% naive definition
  R(t,j,w):-v(j,w),t=j.
  R(t,j,w):-R(t-1,j,w),1<=j<t.
  P[t]=sum[j,w:R(t,j,w)*w].
  S[t,k]=P[t]-P[t-k].
  %% optimized program
  S[t,k]=S[t-1,k]+v[t]-v[t-k-1].
\end{lstlisting}

\remy{TODO: mean, variance}

\subsubsection{Optimization Under Constraints}
APSP (tree), Diameter (tree), MLM (tree)

From Myria: galaxies

\remy{Magic rewrite of same generation and automata also fall into our framework.
  We decided not to include them because they require complex inductive invariants,
  and people can already perform magic-set optimization without synthesis. We'll
  complete these in our next paper!}

\remy{Some additional benchmarks were mentioned in our emails, and we didn't yet
  have time to pursue them: strassen's algorith / matroid / matching, autodiff /
  determinant / inverse.}

\subsection{Results}
