# Supplementary material for: Optimizing Recursive Queries with Program Synthesis
Source: arXiv:2202.10390 source file (2022-02-21)
Supplement: Supplementary file 5 [file appendix-magic-alt-01-03-22.tex]

\section{Examples}

\begin{example}
  \label{ex:hung}  A simple  non-linear query:
  \begin{align*}
    &r_1: & R(x) \cd &  V(x)\\
    &r_2: & R(x) \cd & T(x, y, z) \wedge R(y) \wedge R(z)\\
    &r_3: & Q(x) \cd & R(x) \wedge G(x)
  \end{align*}
  The adorment is $R^+, Q^-$, and the optimized query is:
  \begin{align*}
    &r_4: & Q'() \cd & \\
    &r_5: & R'(y) \cd & R'(x) \wedge T(x,y,z) & \mbox{item~\ref{item:def:magicsets:1} applied to rule $r_2$ and atom $R(y)$} \\
    &r_6: & R'(z) \cd & R'(x) \wedge T(x,y,z) \wedge R(y)  & \mbox{item~\ref{item:def:magicsets:1} applied to rule $r_2$ and atom $R(z)$} \\
    &r_7: & R'(x) \cd & Q() \wedge G(x)   & \mbox{item~\ref{item:def:magicsets:1} applied to rule $r_3$ and atom $R(x)$} \\
    &r_1': & R(x) \cd & R'(x) \wedge V(x)\\
    &r_2': & R(x) \cd & R'(x) \wedge T(x, y, z) \wedge R(y) \wedge R(z)\\
    &r_3': & Q(x) \cd & Q() \wedge R(x) \wedge G(x)
  \end{align*}
\end{example}

\begin{example} \label{ex:triple:tc}
  Consider the following ``triple-transitive closure'':
  \begin{align*}
    \Pi: &r_1: &T(x,y) \cd & E(x,y) \\
         &r_2: &T(x,y) \cd & T(x,u) \wedge T(u,v) \wedge T(v,y) \\
         &r_3: &Q(y) \cd & T(a,y)
  \end{align*}
  We choose to adorn the predicates as follows: $T^{+-}$, $Q^-$.  But
  we will drop the adornments to reduce clutter.  We start by adding
  only the magic predicates:
\begin{align*}
  \Pi_1: & r_4: &Q'() \cd & \\
         & r_5: &T'(u) \cd & T'(x) \wedge T(x,u) & \mbox{item~\ref{item:def:magicsets:1} applied to rule $r_2$ and atom $T(u,v)$}\\
         & r_6: &T'(v) \cd & T'(x) \wedge T(x,u) \wedge T(u,v) & \mbox{item~\ref{item:def:magicsets:1} applied to rule $r_2$ and atom $T(v,y)$}\\
         & r_7: &T'(a) \cd & Q'() & \mbox{item~\ref{item:def:magicsets:1} applied to rule $r_3$ and atom $T(a,y)$}\\
         & r_1: &T(x,y) \cd & E(x,y) \\
         & r_2: &T(x,y) \cd & T(x,u) \wedge T(u,v) \wedge T(v,y) \\
         & r_3: &Q(y) \cd & T(a,y)
\end{align*}
The rewrite in item~\ref{item:def:magicsets:1} applied to rule $r_2$
and atom $T(x,u)$ leads to a trivial rule $T'(x) \cd T'(x)$, which we
removed.  Finally, we apply the transformations in
item~\ref{item:def:magicsets:3}:
\begin{align*}
  \Pi_2: & r_4: &Q'() \cd & \\
         & r_5: &T'(u) \cd & T'(x) \wedge T(x,u)\\
         & r_6: &T'(v) \cd & T'(x) \wedge T(x,u) \wedge T(u,v)\\
         & r_7: &T'(a) \cd & Q'() \\
         & r_8: &T(x,y) \cd & T'(x) \wedge E(x,y) & \mbox{item~\ref{item:def:magicsets:3} applied to rule $r_1$}\\
         & r_9: &T(x,y) \cd & T'(x) \wedge T(x,u) \wedge T(u,v) \wedge T(v,y) & \mbox{item~\ref{item:def:magicsets:3} applied to rule $r_2$} \\
         & r_{10}: &Q(y) \cd & Q'() \wedge T(a,y) & \mbox{item~\ref{item:def:magicsets:3} applied to rule $r_3$}
\end{align*}
\end{example}

\begin{example}
  Consider the reverse-same-generation program:
  \begin{align*}
    r_1: &&  S(x,y) \cd & E(x,y) \\
    r_2: &&  S(x,y) \cd & U(x,p) \wedge S(q,p) \wedge D(y,q) \\
    r_3: &&  Q_1(y) \cd & S(a,y)
  \end{align*}
  To help the reader keep track of the transformations below, we have
  separated the edges into ``up edges'' denoted $U(x,p)$, ``down
  edges'' denoted $D(y,q)$, and horizontal edges denoted $E(x,y)$.
  Our discussion applies immediately to the case when $U=D=E$.  We
  describe here how to derive the magic-set optimized program as a
  sequence of ``modding'' or ``adorments''.

  The first step is create two copies of $S$, the left $Sl$ and the
  right $Sr$.  More precisely, consider the program:
  \begin{align*}
    r_4: && Sl(x,y) \cd & E(x,y) \\
    r_5: && Sr(x,y) \cd & E(x,y) \\
    r_6: && Sl(x,y) \cd & U(x,p)\wedge Sr(q,p) \wedge D(y,q) \\
    r_7: && Sr(x,y) \cd & U(x,p)\wedge Sl(q,p) \wedge D(y,q) \\
    r_8: && Q_2(y) \cd & Sl(a,y)
  \end{align*}

  We prove that new program is equivalent to the previous and, for
  that, we will use the following notation.  If $r, r', \ldots$ are
  rules and $R, R', \ldots$ are relation names, then
  $\Pi(r, r', \ldots; R,R',\ldots)$ denotes the program consisting of
  these rules that returns only the IDB predicates $R, R', \ldots$.
  In this notation the two programs above are $\Pi(r_1,r_2,r_3; Q_1)$
  and $\Pi(r_4,r_5,r_6,r_7,r_8; Q_2)$ respectively.

\begin{proposition}
  $\Pi(r_1,r_2; S,S) \equiv \Pi(r_4,r_5,r_6,r_7; Sl,Sr)$.
\end{proposition}
In other words, if we run rules $r_1, r_2$ and return the pair $(S,S)$
we obtain the same result as running rules $r_4, \ldots, r_7$ and
returning $(Sl,Sr)$.

\begin{proof}
  We use the FGH rule.  The three functions are:
  \begin{align*}
    F(S)\defeq & S' &&\mbox{ where}& S'(x,y)\defeq & E(x,y) \vee \exists p,q(U(x,p) \wedge S(q,p) \wedge D(y,q))\\
    G(S)\defeq & (Sl,Sr) &&\mbox{ where}& Sl(x,y) = Sr(x,y) \defeq & S(x,y)\\
    H(Sl,Sr) \defeq & (Sl',Sr') &&\mbox{ where}& Sl'(x,y)\defeq & E(x,y) \vee \exists p,q(U(x,p) \wedge Sr(q,p) \wedge D(y,q))\\
               &           &&             & Sr'(x,y)\defeq & E(x,y) \vee \exists p,q(U(x,p) \wedge Sl(q,p) \wedge D(y,q))
  \end{align*}
  It is immediate to check that $G(F(S)) = H(G(S))$.
\end{proof}

\begin{corollary}
  $\Pi(r_1,r_2,r_3; Q_1) \equiv \Pi(r_4,r_5,r_6,r_7,r_8; Q_2)$
\end{corollary}

Next, we adorn the IDBs $Sl, Sr, Q_2$ as follows:
$Sl^{+-}, Sr^{-+}, Q_2^-$.  Recall that we are also allowed to reorder
the atoms in each rule: we chose to reorder those in the rule for
$Sr^{-+}$.  The program now becomes:

\begin{align*}
  r_4: && Sl^{+-}(x,y) \cd & E(x,y) \\
  r_5: && Sr^{-+}(x,y) \cd & E(x,y) \\
  r_6: && Sl^{+-}(x,y) \cd & U(x,p)\wedge Sr^{-+}(q,p) \wedge D(y,q) \\
  r_7: && Sr^{-+}(x,y) \cd & D(y,q) \wedge Sl^{+-}(q,p) \wedge U(x,p) \\
  r_8: && Q_2^-(y) \cd & Sl^{+-}(a,y)
\end{align*}

Next, we apply the transformations in Def.~\ref{def:magicsets} and
obtain:

\begin{align*}
  \mbox{item~\ref{item:def:magicsets:1} on $r_6$}: && Sr'(p) \cd & Sl'(x)\wedge U(x,p) \\
  \mbox{item~\ref{item:def:magicsets:1} on $r_7$}: && Sl'(q) \cd & Sr'(y)\wedge D(y,q) \\
  \mbox{item~\ref{item:def:magicsets:1} on $r_8$}: && Sl'(a) \cd & Q_2'()\\
  \mbox{item~\ref{item:def:magicsets:2}}: && Q_2'() \cd &\\
  \mbox{item~\ref{item:def:magicsets:3} on $r_4$}: && Sl^{+-}(x,y) \cd & Sl'(x)\wedge E(x,y) \\
  \mbox{item~\ref{item:def:magicsets:3} on $r_5$}: && Sr^{-+}(x,y) \cd & Sr'(y) \wedge E(x,y) \\
  \mbox{item~\ref{item:def:magicsets:3} on $r_6$}: && Sl^{+-}(x,y) \cd &Sl'(x)\wedge U(x,p)\wedge Sr^{-+}(q,p) \wedge D(y,q) \\
  \mbox{item~\ref{item:def:magicsets:3} on $r_7$}: && Sr^{-+}(x,y) \cd &Sr'(y)\wedge D(y,q) \wedge Sl^{+-}(q,p) \wedge U(x,p) \\
  \mbox{item~\ref{item:def:magicsets:3} on $r_8$}: && Q_2^-(y) \cd & Q_2'(),Sl^{+-}(a,y)
\end{align*}
\end{example}

\section{An Extended FGH-Rule}

Denote by $X, Y, V, W, \ldots$ tuples of relations.  For example
$X = (R, S)$ where $R, S$ are two relations.  If $F(X)$ is a monotone
function whose output has the same type as the input, then we denote
by $\texttt{lfp}(F)$ its least fixpoint.  Equivalently,
$\texttt{lfp}(F)$ is the result of the following program:
\begin{align*}
  & X \leftarrow \emptyset \\
  & \texttt{repeat until no more change}:  \ \ \ X \leftarrow F(X) \\
  & \texttt{return}(X)
\end{align*}

We prove:

\begin{theorem}[Extended FGH-Rule] \label{th:fgh:rule:ext:appendix}
  Consider the following $\name$ programs, where
  $F_1, F_2, G_1, \ldots$ are monotone function.
  \begin{align*}
    \Pi_1: && (X_1,X_2) \cd & (F_1(X_1,X_2),F_2(X_1,X_2)) & \Pi_2: && (Y_1,Y_2) \cd & (H_1(Y_1,Y_2),H_2(Y_1,Y_2))\\
           && (Y_1,Y_2) \cd & (G_1(X_1),G_2(X_2))
\end{align*}
With some abuse, we use $(X_1,X_2) \cd (F_1,F_2)$ to denote the
``rule'' that consists of separate rules $X_1 \cd F_1$ and
$X_2 \cd F_2$; similarly for the other ``rules'' above.
Let $\Psi(X_1,X_2)$ be the following assertion:
\begin{align}
  \Psi(X_1,X_2) \equiv & (F_1(X_1,X_2) \subseteq X_1) \label{eq:psi:appendix}
\end{align}
Assume that the following two identities hold:
\begin{align}
& \forall X_1,X_2:   & G_1(F_1(X_1,X_2))=&H_1(G_1(X_1),G_2(X_2)) \label{eq:fgh:ext:2:appendix} \\
& \forall X_1,X_2, \Psi(X_1,X_2): & G_2(F_2(X_1,X_2)) =  & H_2(G_1(X_1),G_2(X_2)) \label{eq:fgh:ext:1:appendix}
\end{align}
Then $\Pi_1\equiv \Pi_2$.
\end{theorem}

The standard FGH condition for the programs $\Pi_1, \Pi_2$ consists of
the identities~\eqref{eq:fgh:ext:2:appendix}
and~\eqref{eq:fgh:ext:1:appendix} without the precondition $\Psi$.
The theorem allows us to check the first
condition~\eqref{eq:fgh:ext:1:appendix} only under the assumption
$\Psi$.

% that we can apply the FGH-rule under certain weaker assumptions.  To
% see this, denote as follows:
% 
% \begin{align*}
%   \bar X  \defeq & (X_1,X_2) & \bar Y \defeq & (Y_1,Y_2) \\
%   \bar F(\bar X)\defeq  & (F_1(X_1,X_2),F_2(X_1,X_2)) & \bar H(\bar Y) \defeq & (H_1(Y_1,Y_2), H_2(Y_1,Y_2))\\
%  \bar G(\bar X)=&(G_1(X_1),G_2(X_2))
% \end{align*}
% %
% If $\bar G(\bar F(\bar X))=\bar H(\bar G(\bar X))$ holds for all
% $\bar X$, then both identities~\eqref{eq:fgh:ext:2:appendix}
% and~\eqref{eq:fgh:ext:1:appendix} follow.  The theorem states that
% we can weaken the condition for the FGH-rule by
% requiring~\eqref{eq:fgh:ext:1:appendix} to hold only under the
% assumption $\Psi(X_1,X_2)$.

To prove the theorem, we need the following lemma, whose proof can be
found e.g. in~\cite{pods-paper?????}:

\begin{lemma} \label{lemma:nested:fixpoint:appendix}
  Let $F_1(X_1,X_2), F_2(X_1,X_2)$ be two monotone functions,
  s.t. their outputs have the same types a $X_1$ and $X_2$
  respectively.  Denote by:
  \begin{align*}
    X_2^\infty \defeq & \texttt{lfp}(\lambda X_2.F_2(\texttt{lfp}(\lambda X_1.F_1(X_1,X_2)),X_2))
  \end{align*}
Then the following holds:
  \begin{align*}
    \texttt{lfp}(F_1,F_2) = & (\texttt{lfp}(\lambda X_1.F_1(X_1,X_2^\infty)),X_2^\infty)
  \end{align*}
\end{lemma}
The lemma says that the following two programs return the same
value. The first program computes the fixpoint  of $(F_1,F_2)$:
\begin{align*}
 &  (X_1,X_2) \leftarrow (\emptyset,\emptyset) \\
 &  \texttt{repeat until no more change:} \ \ \ \ \ (X_1,X_2)  \leftarrow (F_1(X_1,X_2),F_2(X_1,X_2))\\
 & \texttt{return}(X_1,X_2)
\end{align*}
The second program is:
\begin{align*}
  & X_2 \leftarrow \emptyset \\
  & \texttt{repeat until no more change:} \ \ \ \ \ X_2 \leftarrow  F_2(\texttt{lfp}(\lambda X_1.F_1(X_1,X_2)),X_2)\\
  & \texttt{return}(\texttt{lfp}(\lambda X_1.F_1(X_1,X_2)),X_2)
\end{align*}

\begin{proof} (of Theorem~\ref{th:fgh:rule:ext:appendix}) \yell{For
    the magic-sets proof we need to allow $G_2$ to depend on both
    $X_1, X_2$ but I don't know how to do that in
    Eq.~\eqref{eq:fgh:ext:2:appendix}.}  It helps to visualize the two
  identities
  \eqref{eq:fgh:ext:2:appendix}-\eqref{eq:fgh:ext:1:appendix} as
  commutative diagrams:

\hspace{-4cm}
\parbox{0.4\textwidth}{
\begin{diagram}
  X_1^s & \rTo^{\lambda X_1.F_1(X_1,X_2)} & X_1^{s+1} &(=F_1(X_1,X_2))\\
 \dTo^{G_1} & \eqref{eq:fgh:ext:2:appendix}  & \dTo^{G_1} \\
  Y_1^s & \rTo^{\lambda Y_1.H_1(Y_1,G_2(X_2))} & Y_1^{s+1}&(=H_1(Y_1,G_2(X_2)))
\end{diagram}
}
$\Psi(X_1^t,X_2):$ \hspace{-5cm}
\parbox{0.4\textwidth}{
\begin{diagram}
  X_2^t   & \rTo^{\lambda X_2.F(X_1,X_2)} & X_2^{t+1} &(=F_2(X_1^t,X_2))\\
 \dTo^{G_2}  & \eqref{eq:fgh:ext:1:appendix}    & \dTo^{G_2} &   \\
  Y_2^t  & \rTo^{\lambda Y_2.H_2(G_1(X_1),Y_2)} & Y_2^{t+1}&(=H_2(G_1(X_1),Y_2^t))
\end{diagram}
}

The program $\Pi_1$ in the theorem first computes the fixpoint
$(X_1^\infty,X_2^\infty)=\texttt{lfp}(F_1,F_2)$, then returns
$(G_1(X_1^\infty),G_2(X_2^\infty))$.  Consider the following program
$\Pi_1'$, which returns the IDBs $Y_2^\infty$:
\begin{align*}
  \Pi_1':
  & X_2 \leftarrow \emptyset \\
  & \texttt{repeat until no more change:} \ \ \ \ \ X_2 \leftarrow F_2(\texttt{lfp}(\lambda X_1.F_1(X_1,X_2)),X_2)\\
  & X_2^\infty \leftarrow X_2 \\
  & Y_2^\infty \leftarrow G_2(X_2^\infty)
\end{align*}
By Lemma~\ref{lemma:nested:fixpoint:appendix}, $\Pi_1'$ computes the
same $X_2^\infty$ as $\Pi_1$, therefore both programs compute the same
$Y_2^\infty$.  To compute the quantity $Y_1^\infty$ returned by
$\Pi_1$, we can add the following line to $\Pi_1'$:
\begin{align}
  & Y_1^\infty \leftarrow G_1(\texttt{lfp}(\lambda X_1.F_1(X_1,X_2^\infty)))\label{eq:x1:appendix}
\end{align}

By the same argument, the program $\Pi_2'$ below computes the same
value $Y_2^\infty$ as $\Pi_2$:
\begin{align*}
  \Pi_2':
  & Y_2 \leftarrow \emptyset \\
  & \texttt{repeat until  no more change:} \ \ \ \ \ Y_2 \leftarrow H_2(\texttt{lfp}(\lambda Y_1.H_1(Y_1,Y_2)),Y_2)\\
  & Y_2^\infty \leftarrow Y_2
\end{align*}
Similarly, the quantity $Y_1^\infty$ computed by $\Pi_2$ can be
obtained by adding the following line to $\Pi_2'$:
\begin{align}
   & Y_1^\infty \leftarrow\texttt{lfp}(\lambda Y_1.H_1(Y_1,Y_2^\infty))\label{eq:y1:appendix}
\end{align}

We start by proving that $\Pi_1'\equiv \Pi_2'$.  Denote the following
two functions:
\begin{align*}
  F'(X_2) \defeq & F_2(\texttt{lfp}(\lambda X_1.F_1(X_1,X_2)),X_2) \\
  H'(Y_2) \defeq & H_2(\texttt{lfp}(\lambda Y_1.H_1(Y_1,Y_2)),Y_2)
\end{align*}
With some abuse, we can view both $\Pi_1', \Pi_2'$ as ``datalog''
programs, written as follows:
\begin{align*}
  \Pi_1': && X_2 \cd & F'(X_2) & \Pi_2': && Y_2 \cd & H'(Y_2)\\
          && Y_2 \cd & G_2(X_2)
\end{align*}
Once written this way, they have the same form as the datalog programs
in Eq.~\eqref{eq:p1:p2} (Sec.~\ref{sec:fgh}), and therefore we can
prove their equivalence by using the FGH-rule.  For that, we need to
check the following identity:
\begin{align}
\forall X_2: \ \  G_2(F'(X_2)) = & H'(G_2(X_2)) \label{eq:claim:fp:gp:appendix}
\end{align}
In this equation, both $F'$ and $H'$ contain a fixpoint, and therefore
in order to prove~\eqref{eq:claim:fp:gp:appendix} we will use the
FGH-rule again, as follows.  Fix some IDB values $X_2$, and consider
the following two programs:
\begin{align*}
  \Pi_1'': X_1 \cd & F_1(X_1,X_2) & \Pi_2'': Y_1 \cd & H_1(Y_1,G_2(X_2))\\
           Y_1 \cd & G_1(X_1)
\end{align*}
The assumption~\eqref{eq:fgh:ext:2:appendix} of the theorem represents
precisely the FGH-condition for these two programs, and, therefore,
they are equivalent by the FGH-rule.  Therefore, denoting
\begin{align}
  X_1^\infty \defeq & \texttt{lfp}(\lambda X_1.F_1(X_1X_2)) \label{eq:v:infty:appendix}
\end{align}
the equivalence of $\Pi_1''$ with $\Pi_2''$ can be written as:
$G_1(X_1^\infty)=\texttt{lfp}(\lambda Y_1.H_1(Y_1,G_2(X_2)))$.  Now we
can prove~\eqref{eq:claim:fp:gp:appendix}, and for that we observe:
\begin{align*}
  G_2(F'(X_2)) = & G_2(F_1(X_1^\infty, X_2)) \\
  H'(G_2(X_2)) = & H_2(\texttt{lfp}(\lambda Y_1.H_1(Y_1,G_2(X_2))),G_2(X_2))=H_2(G_1(X_1^\infty),G_2(X_2))
\end{align*}
By the definition of the fixpoint $X_1^\infty$ in
Eq.~\eqref{eq:v:infty:appendix}, the following inclusion holds:
$F_1(X_1^\infty,X_2) \subseteq X_1^\infty$.  Therefore, assertion
$\Psi(X_1^\infty,X_2)$ holds (i.e.~\eqref{eq:psi:appendix} holds),
and, by assumption~\eqref{eq:fgh:ext:1:appendix} of the theorem, we
derive:
\begin{align*}
  G_2(F_2(X_1^\infty,X_2)) =  & H_2(G_1(X_1^\infty),G_2(X_2))
\end{align*}
This proves that $\Pi_1'\equiv \Pi_2'$ i.e. they return the same value
$Y_2^\infty$, and therefore $\Pi_1, \Pi_2$ also return the same value
$Y_2^\infty$.  To prove that $\Pi_1, \Pi_2$ also return the same value
$Y_1^\infty$, consider the two additional
lines,~\eqref{eq:x1:appendix} and~\eqref{eq:y1:appendix}.  These two
lines are precisely the programs $\Pi_1''$ and $\Pi_2''$ above, where
$X_2=X_2^\infty$ and, therefore, they are equivalent.  This completes
the proof of the theorem.
\end{proof}

\section{Proof of the Magic-Set Optimization Using the FGH-Rule}

\dan{I tried to apply Hung's suggestion, to use the theorem from the
  PODS paper.  I got stuck, hopefully it's fixable.}

Consider a datalog program $\Pi$ over IDBs $X=(X_1,X_2,\ldots,X_k)$,
which we write as follows:
\begin{align*}
  \Pi: && X \cd & F(X)
\end{align*}
We further assume that the program returns only one IDB of interest,
e.g. $X_1$, which we will denote for convenience by $Q$ (thus, $Q$ is
$X_1$).  We further assume that $Q$ does not occur in the boy of any
rule.  This is easily enforced by creating a fresh symbol $Q$ and
adding a unique rule $Q \cd \ldots$ that returns whatever is required
by the program.  We illustrate throughout this section with
Example~\ref{ex:triple:tc}.

Fix any adornment (moding) of the IDBs: for each IDB $X_i$, its
adornment is $m_{X_i} \in \set{+,-}^{\text{arity}(X_i)}$.  Our only
restriction is that the adornment of the output predicate is
$m_Q = (-,-,\ldots,-)$.  As before, let $X_i'$ be the {\em magic}
predicate associated to $X_i$, whose variables are the input variables
of $X_i$ (i.e. those adorned with $+$).  Intuitively, we can write
$X_i(\bm u, \bm v)$ and $X_i'(\bm u)$.  We will abbreviate
$X_i \wedge X_i'$ for $X_i(\bm u, \bm v) \wedge X_i'(\bm u)$.

We start by applying the rewrite rule in
items~\ref{item:def:magicsets:1} and ~\ref{item:def:magicsets:2} of
Def.~\ref{def:magicsets}.  After we add these rules the rewritten
program becomes (see the program $\Pi_1$ in
Example~\ref{ex:triple:tc}):
\begin{align*}
  \Pi_1: && Q' \cd &  && \mbox{rewrite rule in item~\ref{item:def:magicsets:2}}\\
         && X' \cd & F'(X', X) && \mbox{rewrite rules in item~\ref{item:def:magicsets:1}}\\
         && X \cd & F(X) && \\
         && Y \cd & X' \wedge X
\end{align*}
where $F'$ is the ICO for the collection of all new rules defined by
item~\ref{item:def:magicsets:1}, and $X \wedge X'$ denotes the
component-wise conjunction:
$(X_1 \wedge X_1', X_2 \wedge X_2', \ldots)$.  We assume that the
predicate returned by $\Pi_1'$ is $Y_1$, i.e. $Q' \wedge Q$.

Trivially, $\Pi$ and $\Pi_1$ compute the same IDBs $X$: the magic IDBs
$X'$ are not used (yet) in the computation of the IDBs $X$.  Moreover,
since $Q'$ has no variables and the first rule sets
$Q' = \texttt{true}$, we have $Y_1=X_1' \wedge X_1 = Q'\wedge Q = Q$.
In other words, $\Pi$ and $\Pi_1$ return the same final output $Q$.

Now we alter the rules for the IDBs $X$, using the rewriting in
item~\ref{item:def:magicsets:1} of Def.~\ref{def:magicsets}, and we
denote by $F''$ the ICO corresponding the modified rules.  The
magic-optimized program is (see also $\Pi_2$ in
Example~\ref{ex:triple:tc}):
\begin{align*}
  \Pi_2: && Q' \cd & \\
         && X' \cd & F'(X',Y) \\
         && Y \cd & F''(X',Y) && \mbox{rewrite rules in item~\ref{item:def:magicsets:3}}
\end{align*}

We prove that $\Pi_1$ and $\Pi_2$ return the same predicates $Y$ (not
just $Y_1$!).  For that we use the extended FGH-rule in
Theorem~\ref{th:fgh:rule:ext:appendix}, making the following
notations:
\begin{align*}
  (F_1,F_2) \defeq & (F',F) & (H_1,H_2) \defeq & (F',F'') \\
  G_1(X') \defeq & X' & G_2(X',X) \defeq & X' \wedge X
\end{align*}

\yell{First bug here:} we need $G_2$ to depend on both $X'$ and $X$,
but in the theorem this does not appear to be possible.  Not sure how
to fix.  For now I will simply assume that $G_2$ may depend on both
$X', X$, and that Eq.~\eqref{eq:fgh:ext:2:appendix} that we need to
check becomes:
\begin{align*}
  G_1(F'(X',X)) = & F'(X',X) = H_1(G_1(X'),G_2(X',X)) = F'(X',X'\wedge X)
\end{align*}

\yell{Second bug here} Surprisingly, this does not seem to hold on
Example~\ref{ex:triple:tc}.  There we have the following:

\begin{align*}
  F'(X',X): & r_4: &Q'() \cd & \\
         & r_5: &T'(z) \cd & T'(x) \wedge T(x,u)\\
         & r_6: &T'(v) \cd & T'(x) \wedge T(x,u) \wedge T(u,v)\\
         & r_7: &T'(a) \cd & Q'() \\
  F'(X',X' \wedge X): & r_4: &Q'() \cd & \\
         & r_5: &T'(z) \cd & T'(x) \wedge T'(x) \wedge T(x,u)\\
         & r_6: &T'(v) \cd & T'(x) \wedge T'(x) \wedge T(x,u) \wedge T'(u) \wedge T(u,v)\\
         & r_7: &T'(a) \cd & Q'() \\
\end{align*}
There is an extra $T'(u)$ in rule $r_6$.

Finally, we check Eq.~\eqref{eq:fgh:ext:2:appendix}:
\begin{align*}
 G_2(X',F(X)) = &  X' \wedge F(X) = F'(X',X'\wedge X)
\end{align*}
This hold by the assumption $F'(X',X) \subseteq X'$.  This is the only
part we know how to prove.  This is easiest seen on
Example~\ref{ex:triple:tc}.  There, $F(X)$ applies rules $r_1, r_2,
r_3$, while  $G_2(X',F(X))$ intersects them with $X'$, in other words
it computes:
\begin{align*}
  r_1':&&& T'(x) \wedge E(x,y) \\
  r_2':&&& T'(x) \wedge T(x,u) \wedge T(u,v) \wedge T(v,y) \\
  r_3':&&& Q'() \wedge T(a,y)
\end{align*}
On the other hand, $F'(X',X'\wedge X)$ represents these rules after
applying the rewritings in item~\ref{item:def:magicsets:3} (i.e. they
become rules $r_8, r_9, r_{10}$), and replacing each $T$ with
$T' \wedge T$:
\begin{align*}
  r_8': &&& T'(x) \wedge E(x,y) \\
  r_9': &&& T'(x) \wedge \left(T'(x) \wedge T(x,u)\right) \wedge \left(T'(u) \wedge T(u,v)\right) \wedge \left(T'(v) \wedge T(v,w)\right) \\
  r_{10}': &&& Q'() \wedge T'(a) \wedge T(a,y)
\end{align*}
These two sets of rules are equivalent, because of the assumption
$\Psi$ which states:
\begin{align*}
  r_4:&& \Rightarrow & Q'()\\
  r_5:&& T'(x)\wedge T(x,u)  \Rightarrow & T'(u) \\
  r_6:&& T'(x) \wedge T(x,u) \wedge T(u,v) \Rightarrow & T'(v) \\
  r_7:&& Q'() \Rightarrow &T'(a)\\
\end{align*}
These implications allow us to ``chase'' the rules $r_1', r_2', r_3'$
above, and they become $r_5', r_6', r_6'$.  This can be generalized.
