# Supplementary material for: Optimizing Recursive Queries with Program Synthesis
Source: arXiv:2202.10390 source file (2022-02-21)
Supplement: Supplementary file 6 [file appendix-magic-oldAppendixC.tex]

\clearpage

\section{Magic Set Optimization}
\label{app:magic:sets}

\newcommand{\au}{\mathtt{aux}}
\newcommand{\fgh}{\textrm{FGH}}

\newcommand{\bA}{\mathbf{A}}
\newcommand{\bB}{\mathbf{B}}
\newcommand{\bC}{\mathbf{C}}

\newcommand{\calO}{\mathcal{O}}
\newcommand{\calP}{\mathcal{P}}
\newcommand{\BP}{B_\mathcal{P}}
\newcommand{\TP}{T_\mathcal{P}}
\newcommand{\MP}{M_\mathcal{P}}
\newcommand{\BO}{B_\mathcal{O}}
\newcommand{\TO}{T_\mathcal{O}}
\newcommand{\MO}{M_\mathcal{O}}
\newcommand{\OT}{\tilde{\mathcal{O}}}
\newcommand{\TOT}{T_{\OT}}


\newcommand{\fl}{\mathtt{flat}}
\newcommand{\up}{\mathtt{up}}
\newcommand{\down}{\mathtt{down}}
\newcommand{\sg}{\mathtt{sg}}
\newcommand{\query}{\mathtt{query}}
\newcommand{\sgbf}{\mathtt{sg^{bf}}}
\newcommand{\sgp}{\mathtt{sg'}}
\newcommand{\isgbf}{\mathtt{input\_sg^{bf}}}
\newcommand{\aux}{\mathtt{aux}}




In \cite{DBLP:conf/birthday/MascellaniP02}, Mascellani and Pedreschi presented a
very elegant correctness proof of the magic set optimization of logic programs. Its main
characteristics are:

\begin{enumerate}
\item applying a declarative style rather than the usual procedural reasoning;
\item allowing arbitrary ``modings'' (i.e., designating input and
output positions in each relation) rather than adornments, which are
usually used to trace the binding of variables in each rule body; and
\item adopting an iterative approach -- considering a single moding at a time rather than
all possible adornments at once.
\end{enumerate}

The actual correctness proof in \cite{DBLP:conf/birthday/MascellaniP02} is heavily
based on the notion of a ``base'' of a logic program. This notion had previously been
used to formalize the idea of ``admissible'' answers to a query, which was usually
done by imposing type constraints on the arguments of a query atom.
In \cite{DBLP:conf/birthday/MascellaniP02}, the relationship between the
original program and its magic set optimization is captured via ``bases'.

In this section, we will show how the
correctness proof of \cite{DBLP:conf/birthday/MascellaniP02}
can be translated into our \fgh-framework. The use of ``bases'' is not needed. However, the definition of the $g$-function
in our \fgh-proof is closely related to the `base'' used in the proof of \cite{DBLP:conf/birthday/MascellaniP02}.
First, we recall some key terminology and notation from
\cite{DBLP:conf/birthday/MascellaniP02}.



\paragraph*{\bf Notation}
As in \cite{DBLP:conf/birthday/MascellaniP02}, we use upper case letters $A,B, \dots $ to denote single literals in a datalog rule and bold face letters $\bA, \bB, \dots$ to denote a (possibly empty) sequence of atoms. Datalog rules are thus of the form
$A \cd \bA$. For given program $\calP$, we write $\BP$, $\TP$, and $\MP$ to denote the Herbrand base of $\calP$, the immediate
consequence operator of $\calP$, and the minimal model of $\calP$, respectively. It is convenient to consider $\MP$ as a set of
ground atoms (rather than, e.g. a collection of relations).
For a single-atom query $Q$, we write $[Q]$ to denote the set of all possible ground instances of $Q$.

%\remy{What does ``all possible instances of $Q$'' mean?
%Is it over all EDBs?}
%
%\reinhard{I have extended ``all instances'' to ``all ground %instances''. Does that clarify things?}

\paragraph*{\bf Modes}
For an $n$-ary relation symbol $p$, a {\em mode\/} for $p$ is a function
%
$$
m_p \colon \{1, \dots, n\} \rightarrow \{+,-\}
$$
with the understanding that $m_p(i) = +$ (respectively  $m_p(i) = -$) means that
$i $ is an input (respectively output) position of $p$.
A more intuitive notation of the moding of a relation symbol
$p$ is in the form $p(m_p(1), \dots, m_p(n))$. In  \cite{DBLP:conf/birthday/MascellaniP02}, this notation is
illustrated by the example $\mathtt{sum}(+,+,-)$, where $\mathtt{sum}$ is a predicate that takes two numbers as input and produces their sum in the third component.

In the sequel, we will assume some fixed moding for
a given program. W.l.o.g., we may assume that, for every relation symbol,
the input positions precede the output positions. Hence, an atom $A$ is of the form $p(\mathbf{u}, \mathbf{v})$ with
input arguments $\mathbf{u}$ and output arguments~$\mathbf{v}$.


\paragraph*{\bf Magic set optimization}
For an atom $A$ of the form $p(\mathbf{u}, \mathbf{v})$, we denote the {\em magic version\/} of $A$ as $A' = p'(\mathbf{u})$
for some fresh predicate symbol $p'$. (Recall that we assume a fixed mode for every relation symbol $p$ in a given program).
Then the magic set transformation can be defined as follows (cf.\ \cite{DBLP:conf/birthday/MascellaniP02}, Definition~3):


\begin{definition}
\label{def:magicsets}
Consider a program $\calP$ together with a single-atom query $Q$. The magic program $\calO$ is obtained from $\calP$ by the
following transformation steps:

\begin{enumerate}
\item \label{item:def:magicsets:1} For every rule $r \colon A \cd \bA$ (with fixed order of the body atoms),
and every atom $B$ in the body of $r$,
let $\bB$ denote the sequence of body atoms
to the left of $B$ and let $\bC$ denote the sequence of body atoms
to the right of $B$, i.e., the rule body $\bA$ is of the form
$\bB, B, \bC$. Then we add a new rule
$B' \cd A', \bB$ to the program;
\item \label{item:def:magicsets:2} add a new single-atom rule $Q' \cd$ ;
\item \label{item:def:magicsets:3} replace each original rule $A \cd \bA$ from $\calP$ by
the new rule $A \cd A', \bA$.
\end{enumerate}
\end{definition}
%
%
As is noted in \cite{DBLP:conf/birthday/MascellaniP02}, the notion of ``modes'' is more general than that of the usual
adornments resulting from a bound/free analysis.
The usual magic set optimization is  obtained  by iterating the above transformation for different modings. The correctness of
the magic set transformation is stated as follows (cf.\ \cite{DBLP:conf/birthday/MascellaniP02}, Theorem 4):


\begin{theorem}
\label{theo:magicsets}
Let $\calP$ be a datalog program with a single-atom query $Q$, and let $\calO$ be the corresponding magic program. Then
the following property holds:
%
%
$$
\MP \cap [Q] = \MO \cap [Q]
$$
\end{theorem}

% add \balance to the first col of the last
% page to remove warning:
% https://tex.stackexchange.com/questions/504955/package-balance-warning-in-acmart
% \balance

In other words, the two programs yield the same answer tuples for query $Q$.

\paragraph*{\bf Correctness proof of the magic set optimization}

Here, we deviate from the proof (based on ``bases'') in \cite{DBLP:conf/birthday/MascellaniP02} and
give a proof based on the \fgh-framework instead.  Let $\MO'$ denote the set of ground instances of magic atoms in $\MO$, i.e.,
atoms of the form $A'$ for atoms $A \in  \BP$.
Finally, let $\OT$ denote the program $\calO$ restricted to the
rules of type (3) in Definition~\ref{def:magicsets}, i.e.,
the rules of the form $A \cd A', \bA$ such that
program $\calP$ contains
a rule $A \cd \bA$.

We define the functions $f,g,h$ on sets of ground atoms, where $f$ and $g$ take as input a set $J \subseteq \BP$ and $h$ takes as
input a set $K \subseteq \BO$.

%
\begin{align*}
    f(J)  &= J \cup  \TP(J) \\
    g(J) &=  \{A \in J \mid A' \in \MO'\} \cup \MO' \\
    h(K)  &= K \cup  \TOT(K)
\end{align*}
%
\hqn{We should probably replace $f(J)= J \cup \TP(J)$ with
$f(J) = \TP(J)$, because $f$ represents datalog so it is monotone,
and thus it is inflationary if we start the sequence from
$\emptyset$. Similarly, replace $h(K)=K\cup \TOT(K)$ with $h(K)=\TOT(K)$ only.
\\
In particular, we want to use $fgh$ to prove that
$g(\TP^\omega (\emptyset)) =
\TOT^\omega (g(\emptyset))$, {\bf not} that
$g((J \cup \TP(J))^\omega (\emptyset)) =
(K\cup \TOT(K))^\omega (g(\emptyset))$.
}
That is, $f$ and $h$ are the (inflationary) immediate consequence operators of programs $\calP$ and $\OT$, respectively.
Function $g$ applied to a set $J \subseteq \BP$ on one hand
restricts $J$ to those atoms which, intuitively, have ``useful'' values in the input positions and, on the other hand, always
adds all the primed atoms contained in $\MO'$.

In the sequel, we tacitly assume that the sets $J$ and $K$
contain all edb-relations. Equivalently, we could assume that
the programs $\calP$ and $\calO$ contain single-atom rules $ A \cd .$ for all all edb-facts $A$ without explicitly
mentioning these additional rules.



\begin{proof}[Proof of the \fgh-property]
Below we show that the following diagram commutes
for arbitrary $J \subseteq \MP$:

% https://q.uiver.app/?q=WzAsNCxbMCwwLCJKIl0sWzIsMCwiSl4qIl0sWzAsMSwiSyJdLFsyLDEsIkteKiJdLFswLDEsImYiXSxbMCwyLCJnIiwyXSxbMiwzLCJoIl0sWzEsMywiZyIsMl1d
\[\begin{tikzcd}
	J && {J^*} \\
	K && {K^*}
	\arrow["f", from=1-1, to=1-3]
	\arrow["g"', from=1-1, to=2-1]
	\arrow["h", from=2-1, to=2-3]
	\arrow["g"', from=1-3, to=2-3]
\end{tikzcd}\]

\bigskip

By showing that the above diagram commutes and by using
$g(\emptyset) = \MO'$,
we conclude that
$g(\TP^\omega (\emptyset)) =
\TOT^\omega (g(\emptyset)) =
\TOT^\omega (\MO')$ holds.
We claim that also $g(\TP^\omega (\emptyset)) = \TO^\omega (\emptyset)$ holds.
To prove this claim
we establish the
equalities $\TO^\omega (\emptyset) = \TO^\omega (\MO') =
\TOT^\omega (\MO')$.


\medskip

%\noindent
``$\TO^\omega (\emptyset) = \TO^\omega (\MO')$'':
recall that $\MO'$ denotes
the set of ground instances of magic atoms in $\MO$. In particular,
$\MO' \subseteq \MO$. In general, for any subset $K \subseteq \MO$,
we have $\TO^\omega (K) = \TO^\omega (\emptyset)$, which is seen as follows:
By the inclusions $\emptyset \subseteq K \subseteq \MO$ and the
monotonicity of $\TO$, we have
$\TO^\omega (\emptyset) \subseteq \TO^\omega (K) \subseteq \TO^\omega (\MO)$.
However, $\MO$ denotes the least fixpoint of program $\calO$
(for the given edb-relations) and, therefore, $\MO = \TO^\omega (\emptyset)$ and
$\TO^\omega (\MO)  = \MO$ hold.
In total, we thus have
$\MO = \TO^\omega (\emptyset) \subseteq \TO^\omega (K) \subseteq \TO^\omega (\MO) = \MO$ and, therefore, all subset inclusions are in fact equalities.


\medskip

%\noindent
``$\TO^\omega (\MO') = \TOT^\omega (\MO')$'':
We show $\TO^n (\MO') = \TOT^n (\MO')$ by induction on $n$.
The inclusion $\supseteq$ is obvious, since program $\calO$ contains all
rules from program $\OT$.
\hqn{
I find it a bit more clear to spell out the details here:
assuming
$\TOT^{n-1}(\MO') \subseteq \TO^{n-1}(\MO')$,
it follows that
\[ \TOT^{n}(\MO') = \TOT(\TOT^{n-1}(\MO'))
    \subseteq \TOT(\TO^{n-1}(\MO'))
    \subseteq \TO(\TO^{n-1}(\MO')) = \TO^n(\MO').
\]
}
For the opposite direction,
let $A \in \TO^{n+1}(\MO') \setminus \TO^n (\MO')$.
We have just seen above that $ \MO = \TO^\omega (\emptyset) =
\TO^\omega (\MO')$ holds. This means that all
primed atoms in $\TO^\omega (\MO')$ are already contained in $\MO'$.
Hence, if $A \in \TO^{n+1}(\MO') \setminus \TO^n (\MO')$,
then $A$ is
derived from  $\TO^n (\MO')$ via a ground instance $A \cd A', \bA$ of some rule in $\calO$.
\hqn{I don't follow the reasoning in the above step. From ``all primed atoms in
$\TO^\omega(\MO')$ are those in $\MO'$", it does not follow that every atom
$A \in \TO^{n+1}(\MO') \setminus \TO^n (\MO')$ is non-prime (for an arbitrary $n$).
In particular, the argument
seems to rely on the assumption that
\[
    \TO^n(\MO') \subseteq \TO^{n+1}(\MO'), \ \ \forall n
\]
or, at least, the assumption was that
the prime-atoms in $\TO^n(\MO')$ are also in $\TO^{n+1}(\MO')$?
Is this obvious?
(The sequence $\TO^n(\emptyset)$ is definitely inflationary, because $\TO$
is monotone; but why is $\TO^n(\MO')$ inflationary?)
I guess the question boils down to whether $\MO' \subseteq \TO(\MO')$ holds?}
By the definition of $\OT$, this rule is also in $\OT$.
Moreover,
by the induction hypothesis, we may assume that all atoms in
$A', \bA$ are contained in $\TOT^n (\MO')$. Hence,
$A$ can also be derived from $\TOT^n (\MO')$ via program $\OT$, i.e.,
$A \in \TOT^{n+1} (\MO')$.

Note that the equality
$\TO^\omega (\MO') = \TOT^\omega (\MO')$
could also be proved
by yet another \fgh-property by defining functions $F,G,H$
as
%
%
\begin{align*}
    F(U)  &= U \cup  \TO(U) \\
    G(U) &=  U \\
    H(V)  &= V \cup  \TOT(V)
\end{align*}
%
%
and  showing that $G(F(U)) = H(G(U))$ holds for every $U$ with
$\MO' \subseteq U \subseteq \MO$.

\smallskip

By the single-atom rule $Q' \cd$ in $\calO$, we
have $Q' \in \MO'$ and, therefore,
$\MP \cap [Q] = g(\MP) \cap [Q]$.
Moreover, as we have just shown,
commutativity of the above diagram implies the
equality
$g(\TP^\omega (\emptyset)) = \TO^\omega (\emptyset)$.
Together with $\MP = \TP^\omega (\emptyset)$ and
$\MO = \TO^\omega (\emptyset)$, we thus get
$\MP \cap [Q] =
\MO \cap [Q]$, i.e., the claim of the theorem.
Hence, it
only remains to show that
$
g(f(J)) = h(g(J))
$
indeed holds for every $J \subseteq \MP$.


\medskip
``$\supseteq$'':
we actually show that this inclusion holds for arbitrary
$J \in \BP$.
\hqn{$J \subseteq \BP$?}
Let $A \in h(g(J))$. The case  $A \in g(J)$ (including the case $A \in \MO'$) is trivial.
So assume $A \not \in g(J)$. Hence, there exists a ground instance
$A \cd A', \bA$ of some rule in $\OT$ such that
$A' \in g(J)$ and $\bA \subseteq g(J) \setminus \MO'$. By the definition of $g$,
all primed atoms in $g(J)$ are in $\MO'$ (thus $A' \in \MO'$) and
all atoms in
$g(J) \setminus \MO'$ are also contained in $J$ (thus $\bA \subseteq J$).
Then $A\in f(J)$ via the ground instance
$A \cd \bA$ of a rule in $\calP$ and
$A \in g(f(J))$ since $A' \in \MO'$.


\medskip

``$\subseteq$'':
we first restrict ourselves to the case $J = \TP^n(\emptyset)$ and prove by induction on $n$ that
$g(\TP^n(\emptyset)) \subseteq \TOT^n (g(\emptyset))$ holds.
%
For the induction begin, this becomes the trivial
inclusion
$g(\emptyset) \subseteq g(\emptyset)$.
%
For the induction step, let
$A \in g(\TP^{n+1}(\emptyset))$.
The case  $A \in g(\TP^{n}(\emptyset))$ (including
the case $A \in \MO'$) is trivial.
\hqn{I assume the reasoning goes like this:
$A \in g(\TP^{n}(\emptyset))$ implies
$A \in h(g(\TP^{n}(\emptyset))$ because $h$ is inflationary?
But, if we set $h = \TOT$ and we start the sequence from $g(\emptyset)$ (instead of starting
from $\emptyset$), how do we show that the sequence $\TOT^n(g(\emptyset))$ is
inflationary?
For this assumption to hold, we must show somewhere that
$\TOT(g(\emptyset)) \subseteq \TOT^2(g(\emptyset))$
for the motonotinicty of $\TOT$ to take over.
Or, the induction can start earlier by showing that
$\MO' = g(\emptyset) \subseteq \TOT(g(\emptyset))$.
I assume this holds trivially because we keep all prime-atoms the same (as $\MO'$)
in the $\TOT$-program, treating them as EDBs?
%(We can also set $h(K) = K \cup \TOT(K)$, in which case $h$ would be inflationary but that
%does not seem to be what we want.)
}
So assume  $A \not\in g(\TP^{n}(\emptyset))$.
Hence, there exists a ground instance $A \cd \bA$ of some rule in $\calP$ such that
$\bA \subseteq \TP^{n}(\emptyset)$ and,
moreover, $A' \in \MO'$.
By the induction hypothesis, we assume that
$g(\TP^{n}(\emptyset)) \subseteq \TOT^n (g(\emptyset))$ holds. Moreover, recall from the considerations at
the beginning of the proof that
$\TOT^\omega(\MO') = \MO$ holds. Hence, we  have
$\TOT^n (g(\emptyset)) \subseteq \MO$.
\hqn{I guess this conclusion comes from the same inflationary assumption
of the $\TOT^n(g(\emptyset))$ sequence.
}

\reinhard{Apart from a minor typo ($\in$ vs.\ $\subseteq$), 
all of Hung's comments are related to the the question 
if the various ICOs are
inflationary or not. I admit, this is indeed a mess. 
Unless we explicitly request that the ICOs are inflationary
(e.g.: defining $h(K) = K \cup \TOT(K)$ as I tried), 
we cannot assume that 
$M'_{\calO} \subseteq \TO(M'_{\calO})$ or
$M'_{\calO} \subseteq \TOT(M'_{\calO})$ 
holds. \\
%
In Remy's proof in Appendix D, this problem of inflationary ICOs disappears since we are assuming $R_{\texttt{copy}}$ and $R'_o$ (the analogue of $M'_{\calO})$ as EDBs. I think this is the way to go: much more elegant and clearer.}

We claim that $\bA \subseteq g(\TP^{n}(\emptyset))$ holds. The proof of this claim is by induction on the
atoms in $\bA$. For the induction begin, $\bA$ is the empty sequence and the claim holds trivially.
For the induction step, let $A \cd \bA$ be of the form $A \cd \bB, B, \bC$. By the induction
hypothesis, assume that $\bB \subseteq g(\TP^{n}(\emptyset))$ holds.
In total, we thus have
$\bB \subseteq g(\TP^{n}(\emptyset)) \subseteq \TOT^n (g(\emptyset)) \subseteq \MO$.
%
We have to show that $B \in g(\TP^{n}(\emptyset))$ holds.

By the magic transformation in Definition~\ref{def:magicsets},
program $\calO$
contains a rule with ground instance $B' \cd A', \bB$.
We are assuming $A' \in \MO'$ and,
by the induction hypothesis, we have $\bB \subseteq  g(\TP^{n}(\emptyset))$
with $g(\TP^{n}(\emptyset)) \subseteq \TOT^n (g(\emptyset)) \subseteq \MO$.
Hence,
by the rule $B' \cd A', \bB$,
we have $B' \in \MO$ and, therefore, also $B' \in \MO'$.
Together with $B \in \TP^{n}(\emptyset)$,
it follows that
$B \in g(\TP^{n}(\emptyset))$ holds.
This concludes the induction proof
of the claim that $\bA \subseteq g(\TP^{n}(\emptyset))$ holds.

By the construction of the magic program in Definition~\ref{def:magicsets},
we know that $\calO$ contains a rule with ground instance
$A \cd A', \bA$ and,
by the definition of $\OT$, this rule is also
contained in $\OT$.
By $A' \in \MO' \subseteq
\TOT^n (g(\emptyset))$
and
(as we have just proved) $\bA \subseteq
g(\TP^{n}(\emptyset)) \subseteq \TOT^n (g(\emptyset))$,
atom $A$ is also contained in $\TOT^{n+1} (g(\emptyset))$.

It remains to extend the inclusion $g(f(J)) \subseteq h(g(J))$
from the case $J = \TP^{n}(\emptyset)$ for some $n \geq 0$ to arbitrary
$J \subseteq \MP$.
We may now use the fact that $g(\TP^{n}(\emptyset)) \subseteq \TOT^n (g(\emptyset))$ holds for every $n \geq 0$. Hence,
together with $\TOT^n (g(\emptyset)) \subseteq \MO$,
we have $g(J) \subseteq \MO$ for every $J \subseteq \MP$.
Then the proof of $g(f(J)) \subseteq h(g(J))$ for
arbitrary $J \subseteq \MP$ follows exactly the same lines as
for the case $J = \TP^{n}(\emptyset)$. That is,
consider $A \in g(f(J))$, such that
$A \not\in g(J)$ and, hence,  $A \not\in \MO'$.
Then there exists a ground instance $A \cd \bA$ of some rule in $\calP$ such that
$\bA \subseteq J$ and, moreover, $A' \in \MO'$.
Then we prove by induction on $\bA$ that also $\bA \subseteq g(J)$ holds. For the induction step, let $A \cd \bA$ be of the form $A \cd \bB, B, \bC$. By the induction
hypothesis, we may assume that $\bB \subseteq g(J)$.
Moreover, $\calO$ contains a rule with ground instance
$B' \cd A', \bB$. Now we use the fact $g(J) \subseteq \MO$
and conclude that $B' \in \MO$ and, therefore, also
$B' \in \MO'$. The remainder of the proof can be taken over
literally from the case $J = \TP^{n}(\emptyset)$.
\end{proof}


We now illustrate the above formulation of the magic set transformation
and its correctness proof by the ``same-generation'' program.
Suppose that we
are given a graph with
2 kinds of edges $\fl$ (for horizontal connections) and $\up$
(for vertical connections) and that we are interested in all vertices from the
``same generation'' as some given vertex $\mathtt{a}$. Then the program together with
the corresponding query are defined as follows:

\medskip

\noindent
\texttt{Program} $\calP$: \\
$\mathtt{\sg(x,y)}$ :- $\mathtt{\fl(x,y)}$. \\
$\mathtt{\sg(x,y)}$ :- $\mathtt{\up(x,x_1), \sg(x_1,y_1), \up(y,y_1)}$. \\
with single-atom query  $\mathtt{\sg(a,y)}$


\medskip

\noindent
Let us choose the mode $\sg(+,-)$ for the only idb-predicate of the program.
As we will see below, modes for the edb-predicate are irrelevant.
By step 1 of the magic transformation in Definition \ref{def:magicsets}, we get the following rule:

\medskip

\noindent
$\mathtt{\sgp(x_1)}$ :- $\mathtt{\sgp(x), \up(x,x_1)}$.

\medskip

\balance
\noindent
Note that, in principle, step 1 as defined in Definition~\ref{def:magicsets}
(and in \cite{DBLP:conf/birthday/MascellaniP02}) would also produce
rules with head atom $\up'$. However, since edb atoms never occur in a
rule head, step 3 of the magic transformation would never use a primed
edb-predicate in the body of any rule.
Hence, the primed version of edb-predicates would have
no effect at all on the query atom and can, therefore, safely be omitted.

Now consider step 2 of the magic set transformation in
Definition~\ref{def:magicsets}. It produces the following rule:

\medskip

\noindent
$\mathtt{\sgp(a)}$ :- .

\medskip

Finally, by step 3, we replace the original rules with head predicate
$\sg$ by the following rules:

\medskip

\noindent
$\mathtt{\sg(x,y)}$ :- $\mathtt{\sgp(x), \fl(x,y)}$. \\
$\mathtt{\sg(x,y)}$ :- $\mathtt{\sgp(x),\up(x,x_1), \sg(x_1,y_1), \up(y,y_1)}$.

\medskip

So, in total, we get the following optimized program $\calO$:

\medskip

\noindent
\texttt{Program} $\calO$: \\
$\mathtt{\sgp(x_1)}$ :- $\mathtt{\sgp(x),\up(x,x_1)}$. \\
$\mathtt{\sgp(a)}$ :- .   \\
$\mathtt{\sg(x,y)}$ :- $\mathtt{\sgp(x), \fl(x,y)}$. \\
$\mathtt{\sg(x,y)}$ :- $\mathtt{\sgp(x),\up(x,x_1), \sg(x_1,y_1), \up(y,y_1)}$. \\
with single-atom query  $\mathtt{\sg(a,y)}$


\medskip
\noindent
Note that this is exactly the program that we would get by the usual magic set transformation based on adornments (see e.g., \cite{DBLP:books/aw/AbiteboulHV95})
by considering the adornment $\sgbf$ for the only idb-predicate $\sg$ and renaming
the ``magic predicate'' $\sgp$ to $\isgbf$. Moreover, by way of a minor optimization,
one could define an auxiliary relation $\au$ for the atom sequence  $\mathtt{\sgp(x),\up(x,x_1)}$ to avoid the need to compute this join twice (in the first and last rules above).




\begin{example}
\label{ex:magic:sets}
Suppose that we want to apply the programs $\calP$ and $\calO$ to the graph
$G$ with the following $\fl$ and $\up$ edges:


\bigskip

\begin{center}
\begin{tabular}{c|c}
\multicolumn{2}{c}{$\fl$:} \\
\hline
\texttt{b} & \texttt{e} \\
\texttt{c} & \texttt{f} \\
\texttt{f} & \texttt{c}
\end{tabular}
%
\hspace{50pt}
%
\begin{tabular}{c|c}
\multicolumn{2}{c}{$\up$:} \\
\hline
\texttt{a} & \texttt{b} \\
\texttt{a} & \texttt{c} \\
\texttt{b} & \texttt{c} \\
\texttt{d} & \texttt{e} \\
\texttt{e} & \texttt{f}
\end{tabular}
\end{center}

\bigskip

We get the following minimal models of
$\calP$ and $\calO$ over the input database $G$:
%
{\small
\begin{align*}
    \MP  &= G \cup \{\mathtt{\sg(a,d)},
\mathtt{\sg(a,e)},
\mathtt{\sg(b,e)},
\mathtt{\sg(c,f)},
\mathtt{\sg(d,a)},
\mathtt{\sg(e,b)},
\mathtt{\sg(f,c)}\} \\
%
\MO &= G \cup \{\mathtt{\sgp(a)},
\mathtt{\sgp(b)}, \mathtt{\sgp(c)},
\mathtt{\sg(a,d)},
\mathtt{\sg(a,e)},
\mathtt{\sg(b,e)}
\mathtt{\sg(c,f)} \}
%
\end{align*}
} % end of \small
%
That is, in both cases, the instances of the query atom $\mathtt{\sg(a,y)}$ are
$\{\mathtt{\sg(a,d)},
\mathtt{\sg(a,e)} \}$.

Let us also check one application of the
\fgh-rule. Suppose that we choose $J \subseteq \MP$ with $J = \{
\mathtt{\sg(b,e)}$,
$\mathtt{\sg(c,f)}$,
$\mathtt{\sg(f,c)}$. Note that this would be the result of one application of $\TP$ to the input database $G$. We now verify that, for this set $J$, the equality $g(f(J)) = h(g(J))$ holds. First note that we have $\MO' = \{\mathtt{\sgp(a)},
\mathtt{\sgp(b)},
\mathtt{\sgp(c)}
\}$. Then we get:
%
%
\begin{align*}
    J^* &= f(J) = J \cup
    \{\mathtt{\sg(a,d)},\mathtt{\sg(a,f)},
    \mathtt{\sg(e,b)} \} \\
    K^*  &= g(J^*) = \MO' \cup G \cup
    \{\mathtt{\sg(b,e)},\mathtt{\sg(c,f)},
    \mathtt{\sg(a,d)},\mathtt{\sg(a,f)} \} \\
    K  &= g(J) = \MO' \cup G \cup
    \{\mathtt{\sg(b,e)},\mathtt{\sg(c,f)} \\
    K^*  &= h(K) = K \cup
    \{\mathtt{\sg(a,d)},\mathtt{\sg(a,f)} \}
%
%
\end{align*}

The two ways of computing $K^*$ as $K^* = g(f(J))$
and as $K^* = h(g(J))$, respectively, yield the same result. Of course, as was shown in the proof of Theorem \ref{theo:magicsets}, this is the case for  any $J$.
\end{example}

\clearpage
